# Supplementary material for: Modelling COVID-19 -- I A dynamic SIR(D) with application to Indian data
Source: arXiv:2009.05044 source file (2020-09-10)
Supplement: Supplementary file 1 [file MB_AB_COVID19_Suppl_figures.pdf]

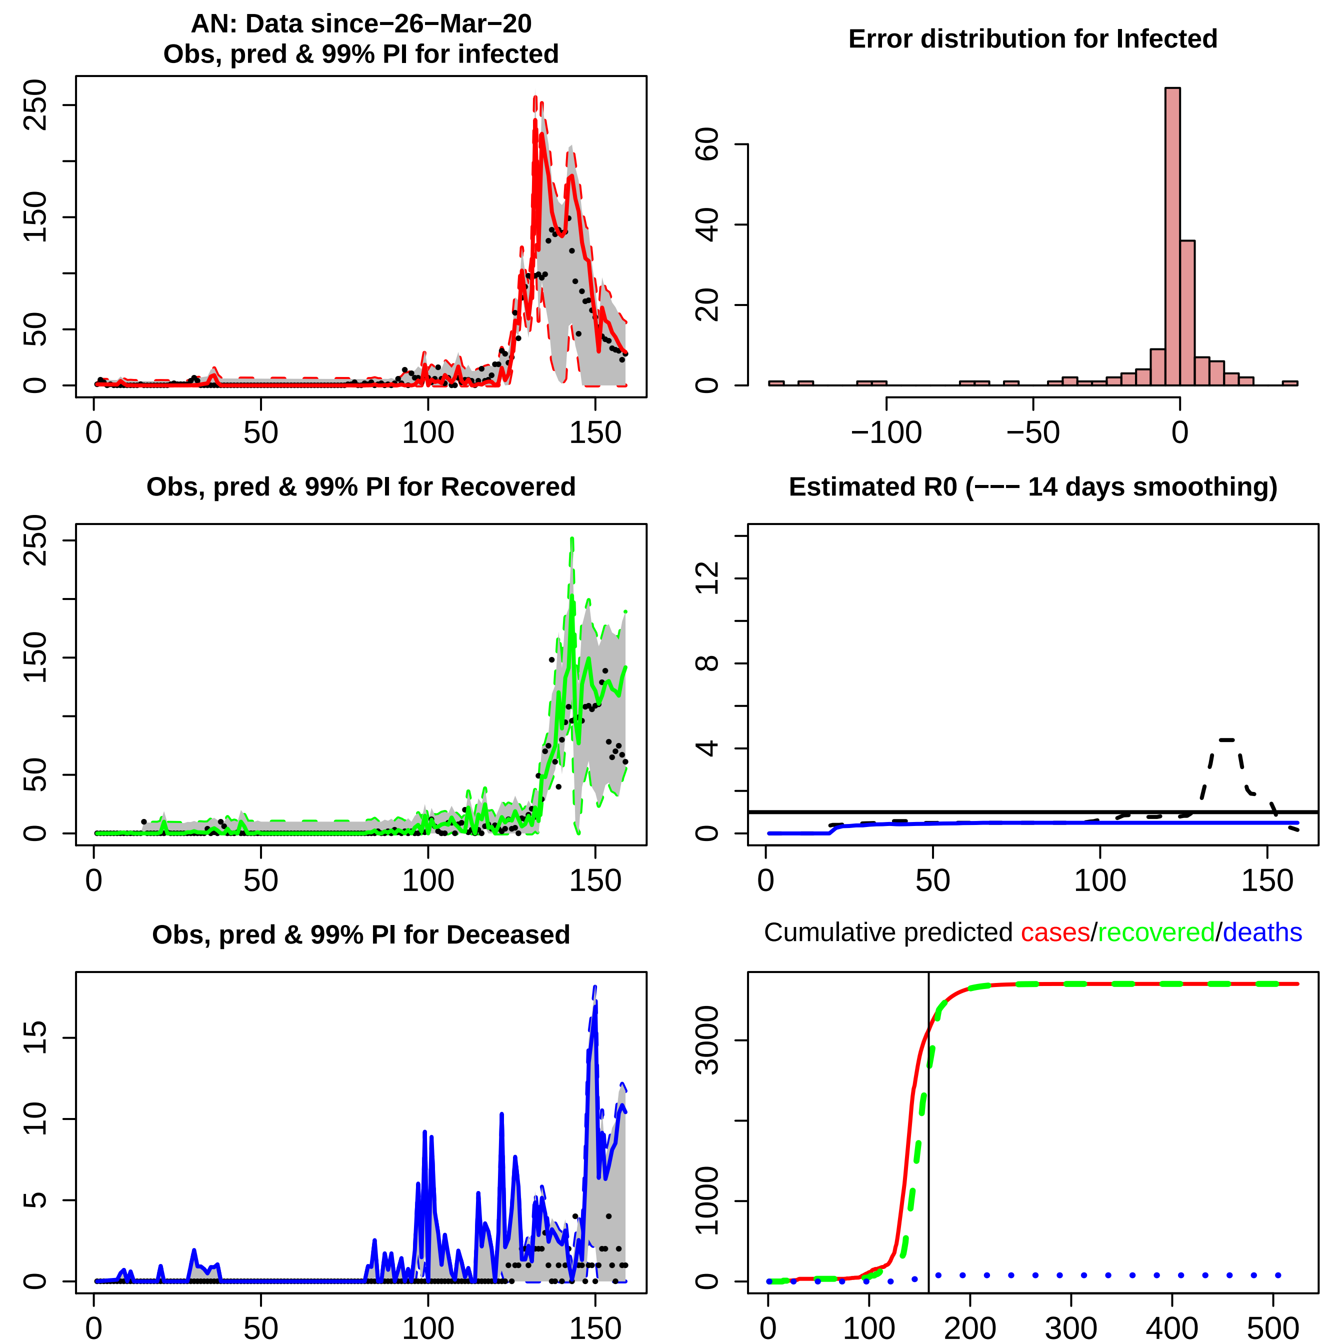
AN: Data since−26−Mar−20
Obs, pred & 99% PI for infected
Error distribution for Infected
Obs, pred & 99% PI for Recovered
Estimated R0 (−−− 14 days smoothing)
Obs, pred & 99% PI for Deceased
Cumulative predicted cases/recovered/deaths
0
50
100
150
250
−100
−50
20
40
60
4
8
12
5
10
15
1000
3000
200
300
400
500

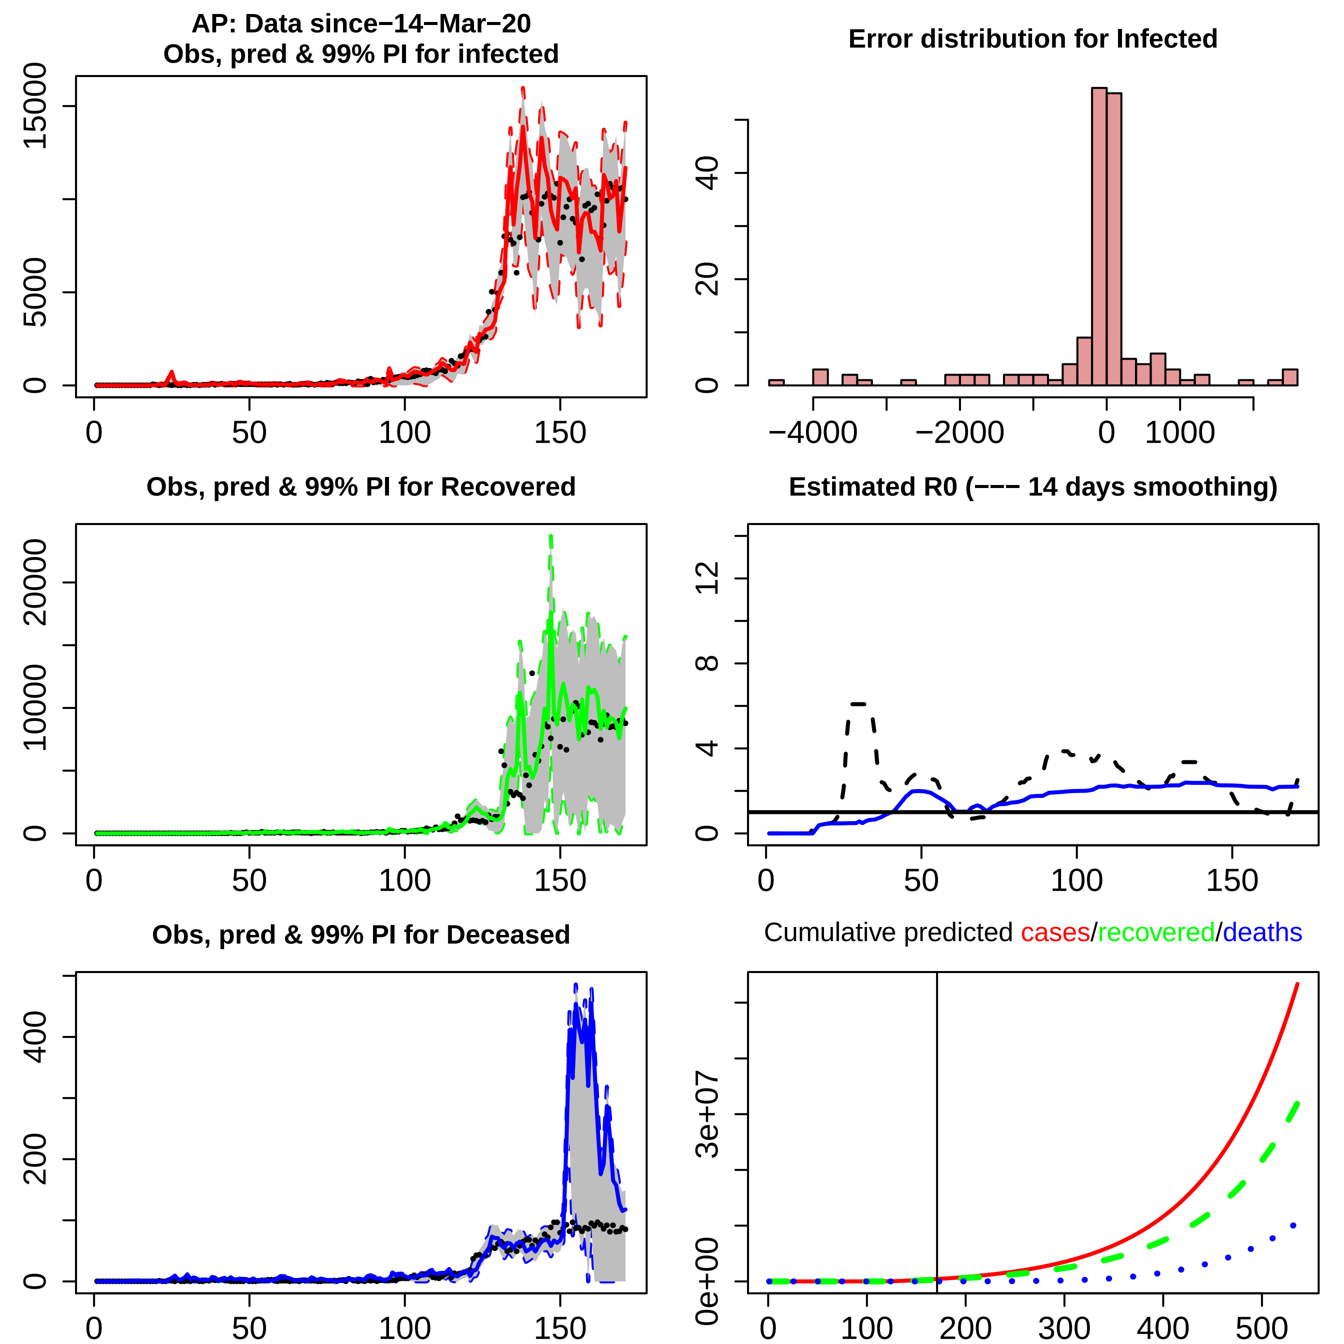
AP: Data since−14−Mar−20
Obs, pred & 99% PI for infected
15000
5000
0
0
50
100
150
Error distribution for Infected
40
20
0
−4000
−2000
0
1000
Obs, pred & 99% PI for Recovered
20000
10000
0
0
50
100
150
Estimated R0 (−−− 14 days smoothing)
12
8
4
0
0
50
100
150
Obs, pred & 99% PI for Deceased
400
200
0
0
50
100
150
Cumulative predicted cases/recovered/deaths
3e+07
0e+00
0
100
200
300
400
500

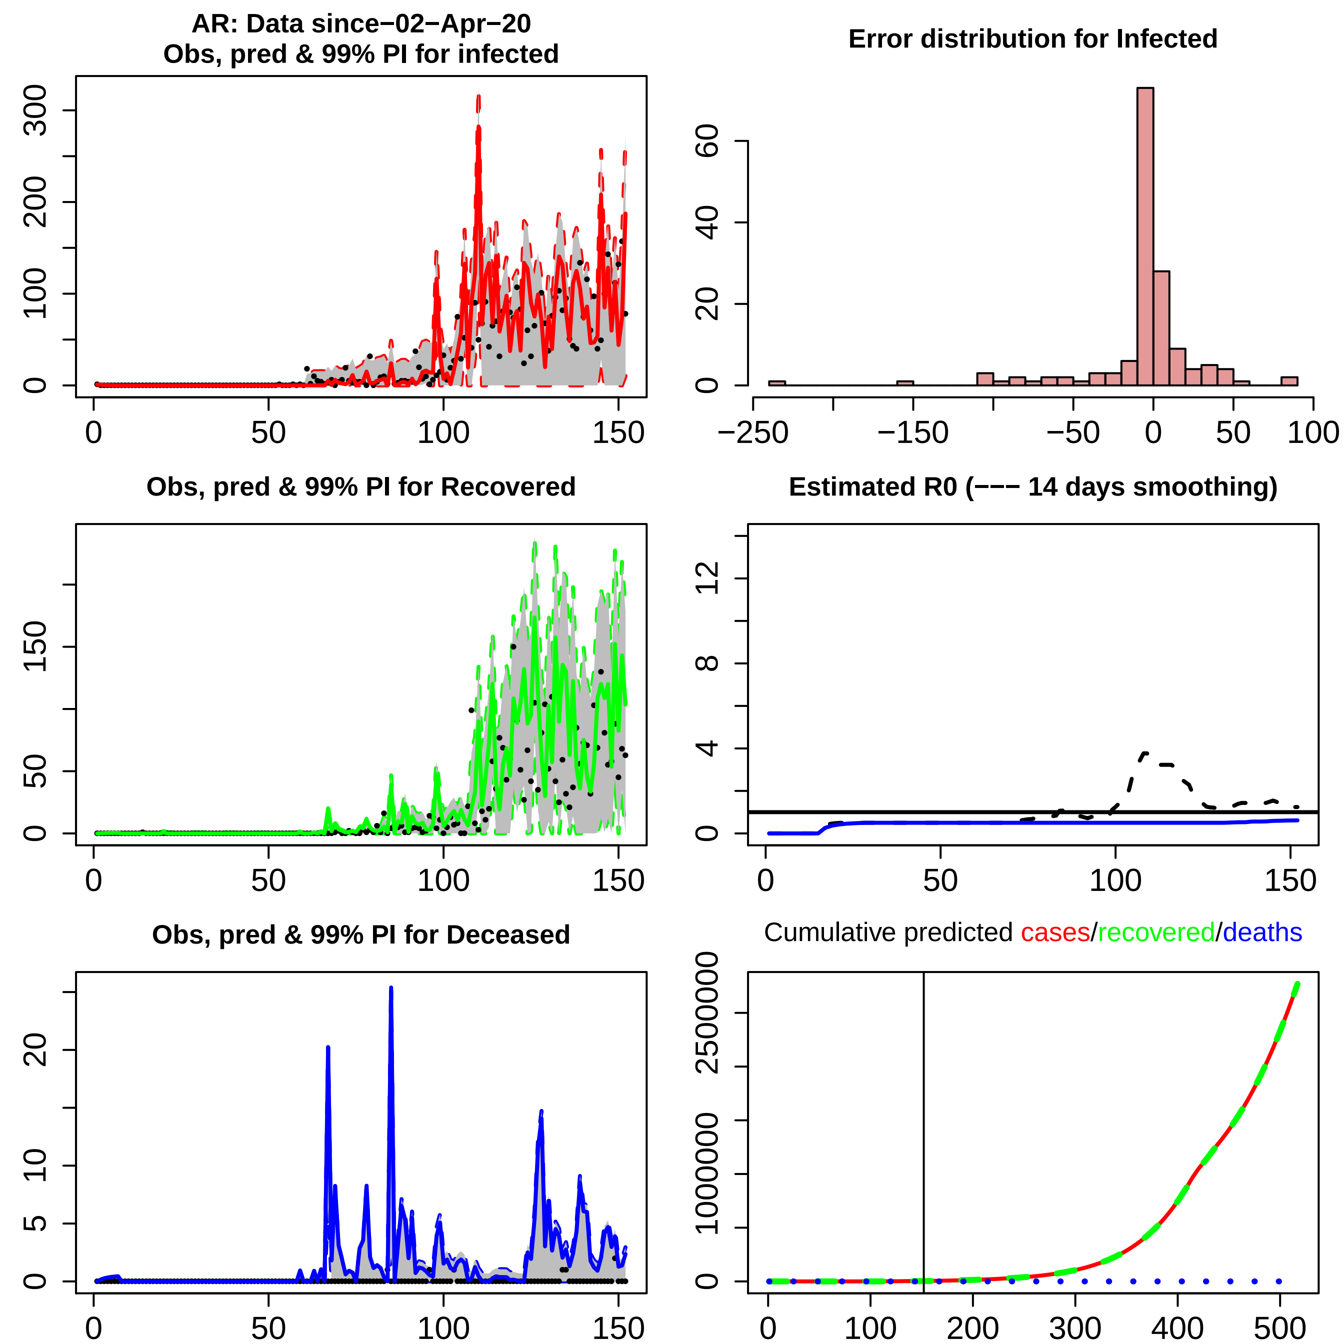
AR: Data since−02−Apr−20
Obs, pred & 99% PI for infected
Error distribution for Infected
Obs, pred & 99% PI for Recovered
Estimated R0 (−−− 14 days smoothing)
Obs, pred & 99% PI for Deceased
Cumulative predicted cases/recovered/deaths

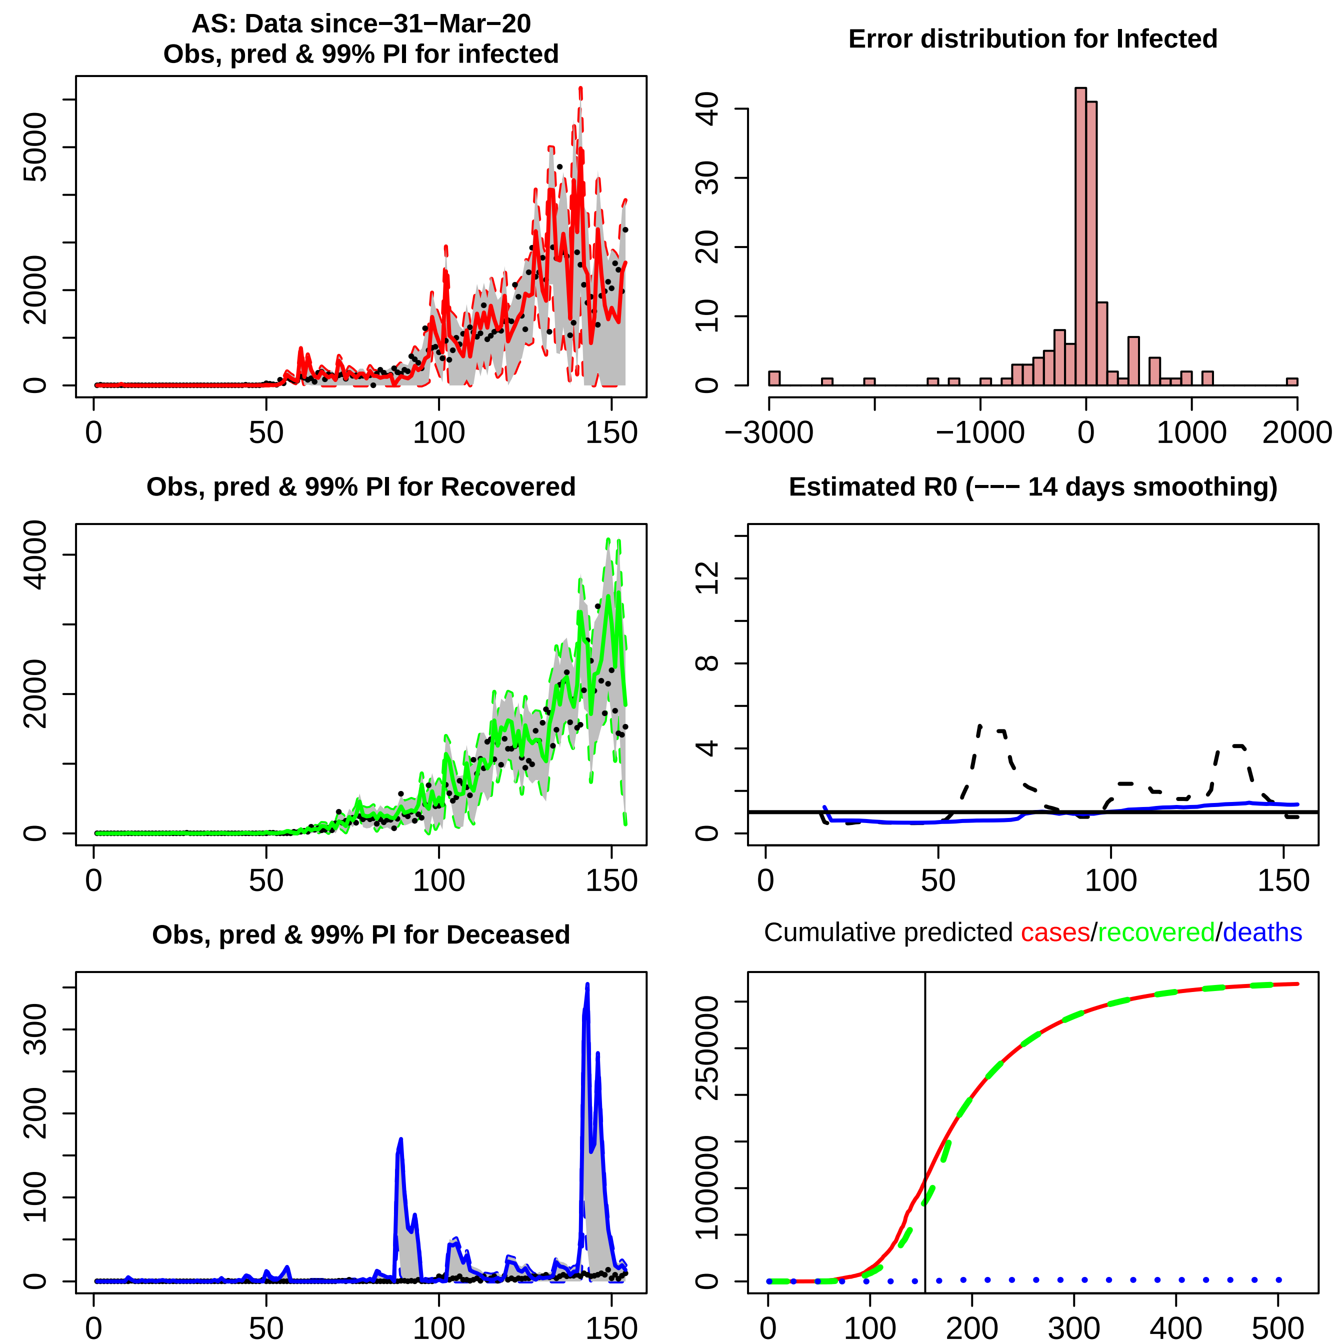
AS: Data since−31−Mar−20
Obs, pred & 99% PI for infected
Error distribution for Infected
Obs, pred & 99% PI for Recovered
Estimated R0 (−−− 14 days smoothing)
Obs, pred & 99% PI for Deceased
Cumulative predicted cases/recovered/deaths

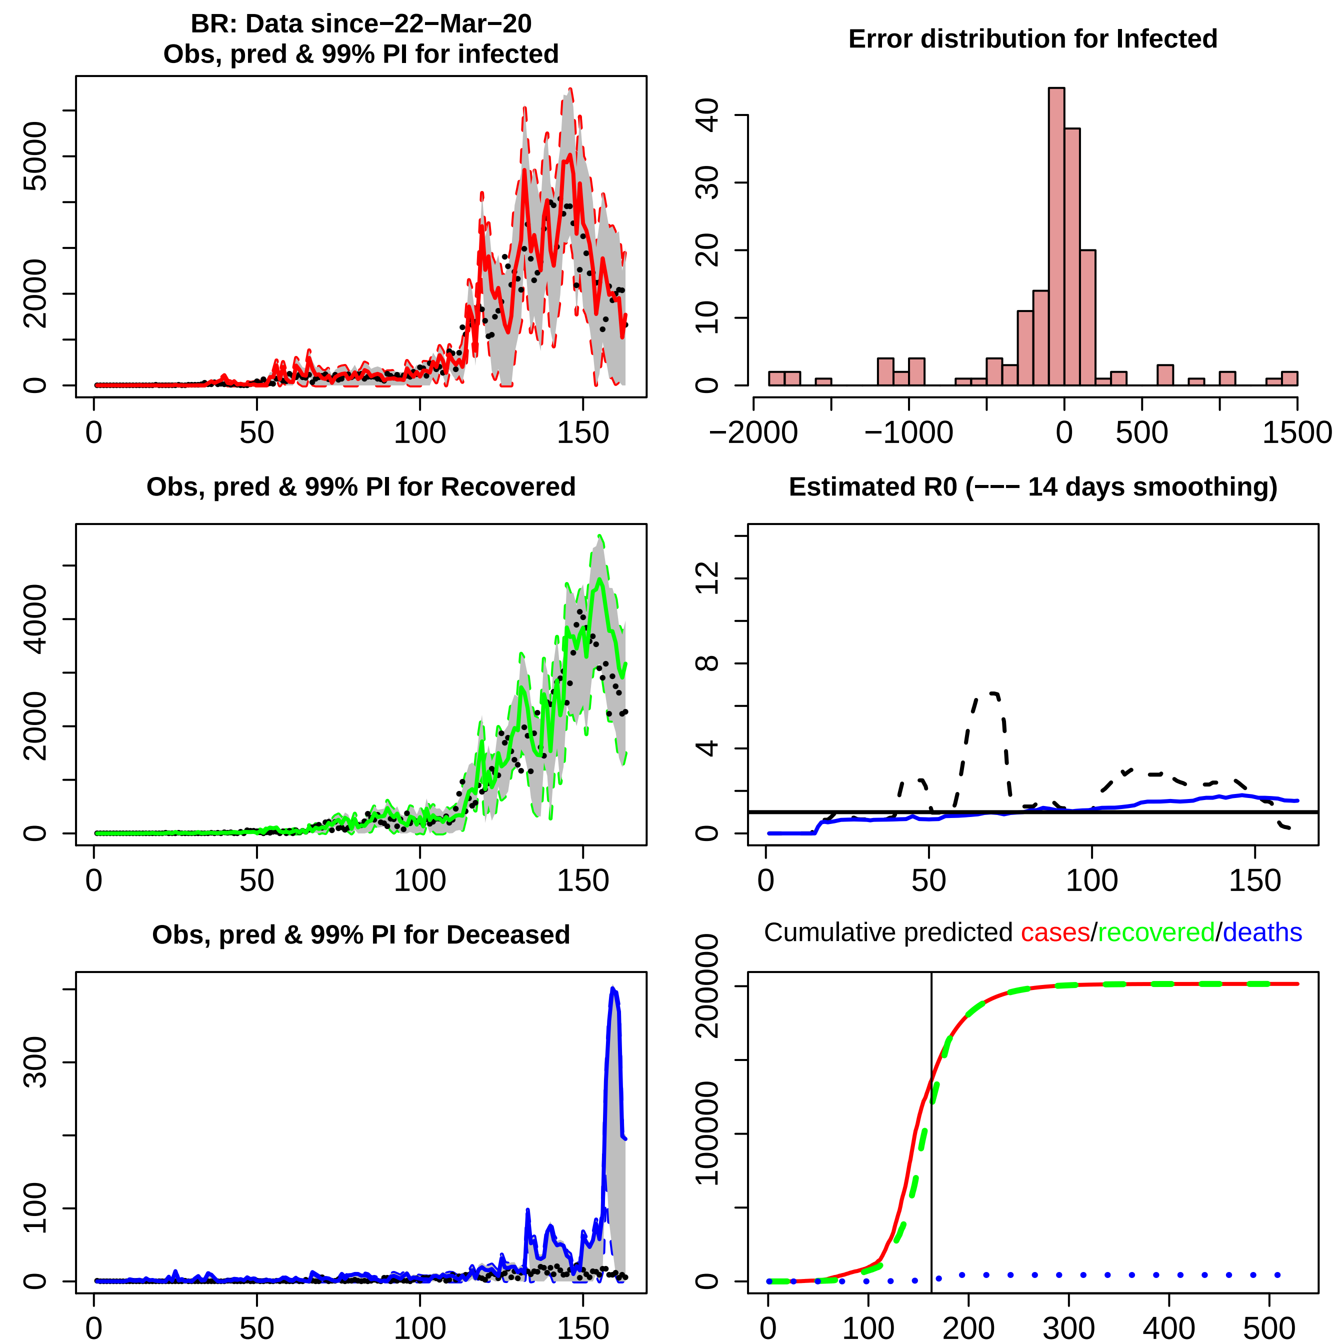
BR: Data since−22−Mar−20
Obs, pred & 99% PI for infected
0
2000
5000
0
50
100
150
Error distribution for Infected
0
10
20
30
40
−2000
−1000
0
500
1500
Obs, pred & 99% PI for Recovered
0
2000
4000
0
50
100
150
Estimated R0 (−−− 14 days smoothing)
0
4
8
12
0
50
100
150
Obs, pred & 99% PI for Deceased
0
100
300
0
50
100
150
Cumulative predicted cases/recovered/deaths
0
100000
200000
0
100
200
300
400
500

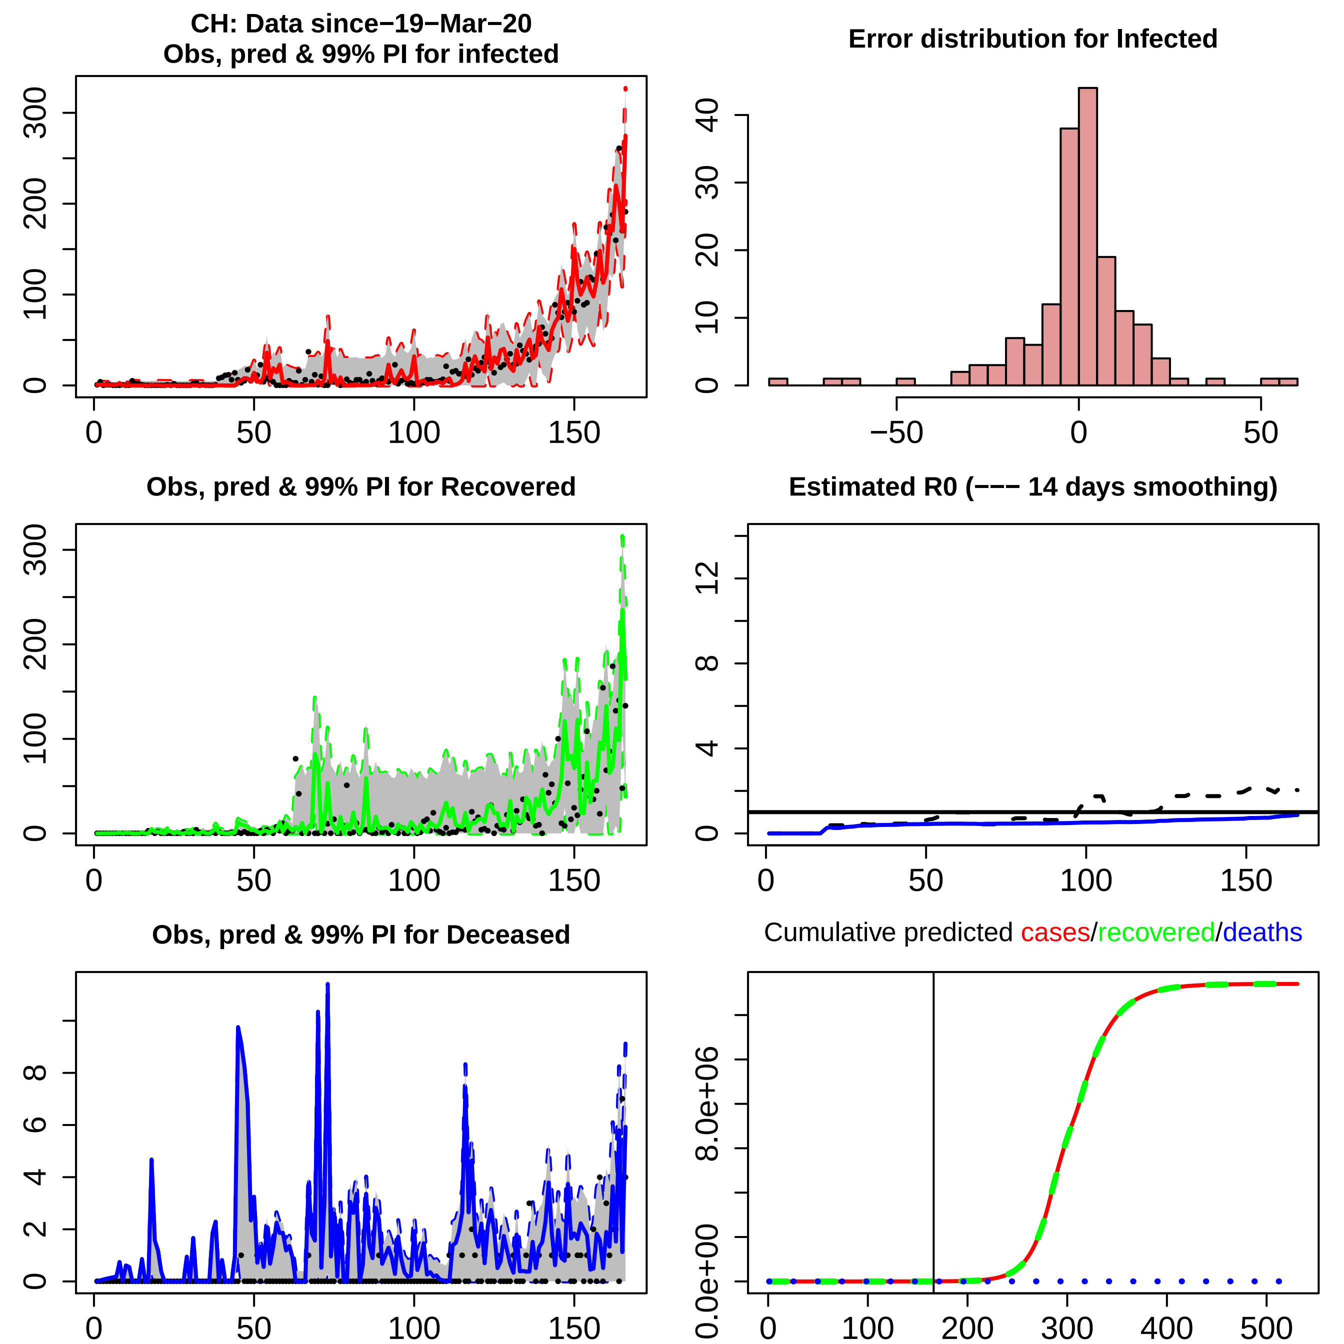
CH: Data since−19−Mar−20
Obs, pred & 99% PI for infected
0 100 200 300
0 50 100 150
Error distribution for Infected
0 10 20 30 40
−50 0 50
Obs, pred & 99% PI for Recovered
0 100 200 300
0 50 100 150
Estimated R0 (−−− 14 days smoothing)
0 4 8 12
0 50 100 150
Obs, pred & 99% PI for Deceased
0 2 4 6 8
0 50 100 150
Cumulative predicted cases/recovered/deaths
0.0e+00 8.0e+06
0 100 200 300 400 500

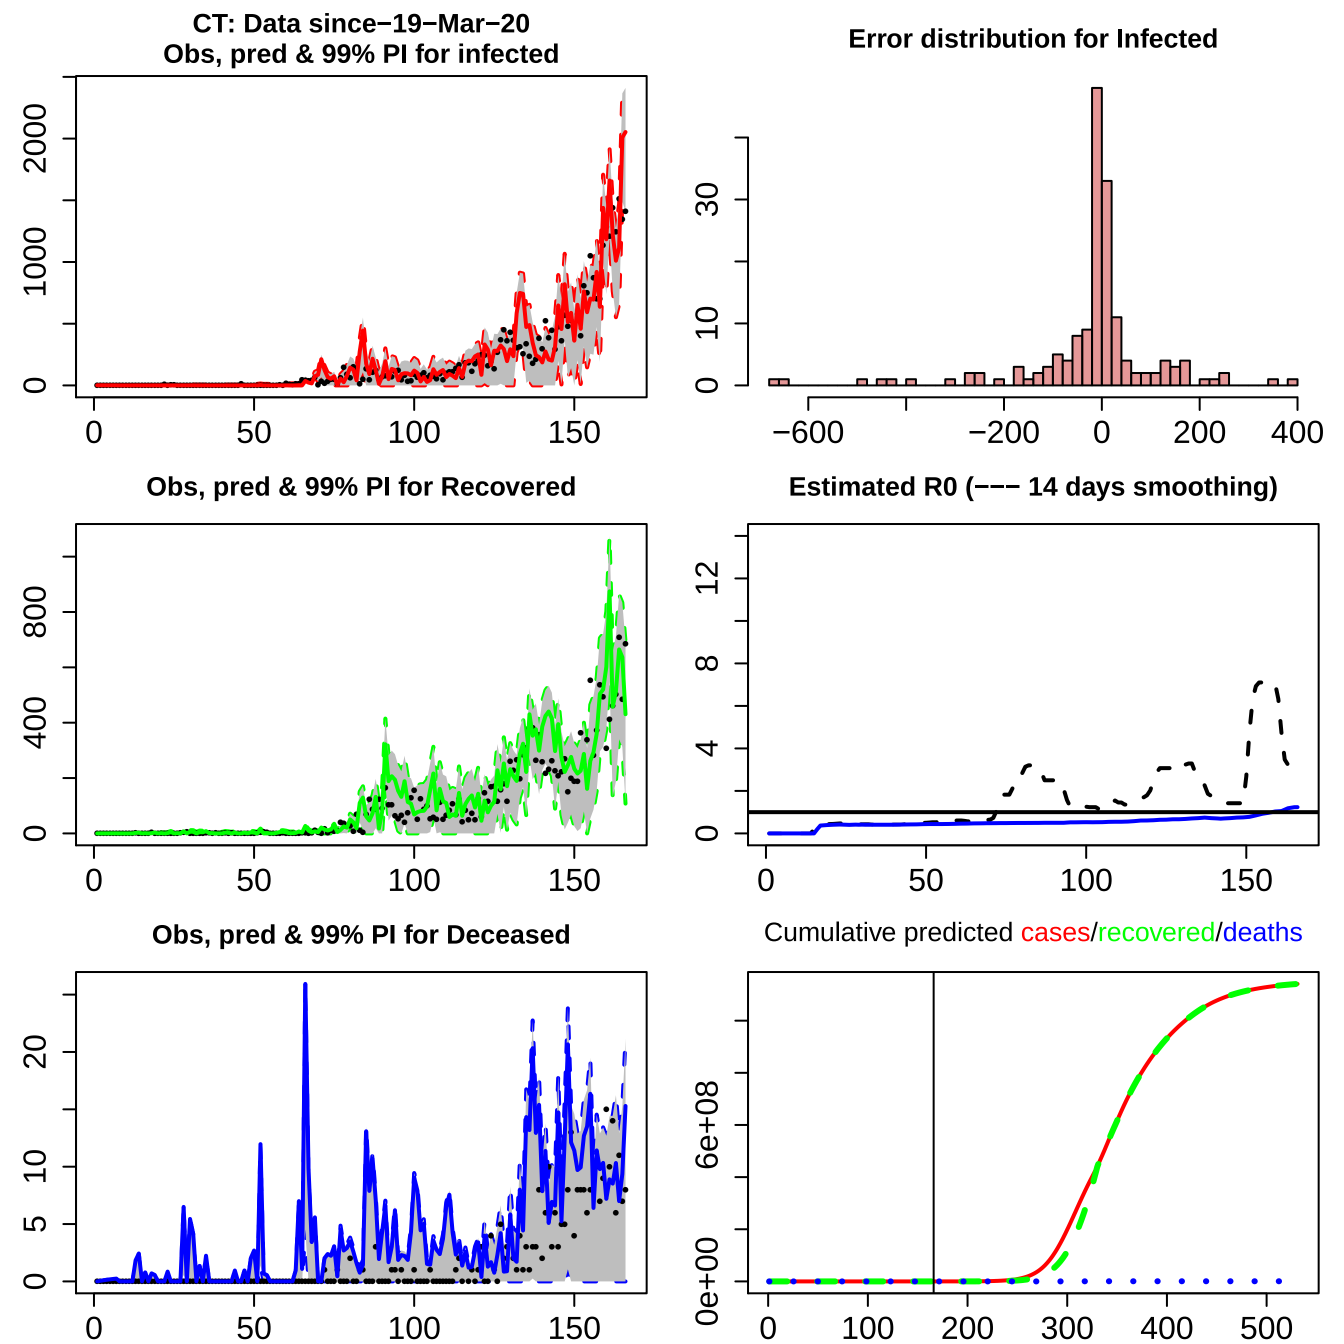
CT: Data since−19−Mar−20
Obs, pred & 99% PI for infected
Error distribution for Infected
Obs, pred & 99% PI for Recovered
Estimated R0 (−−− 14 days smoothing)
Obs, pred & 99% PI for Deceased
Cumulative predicted cases/recovered/deaths

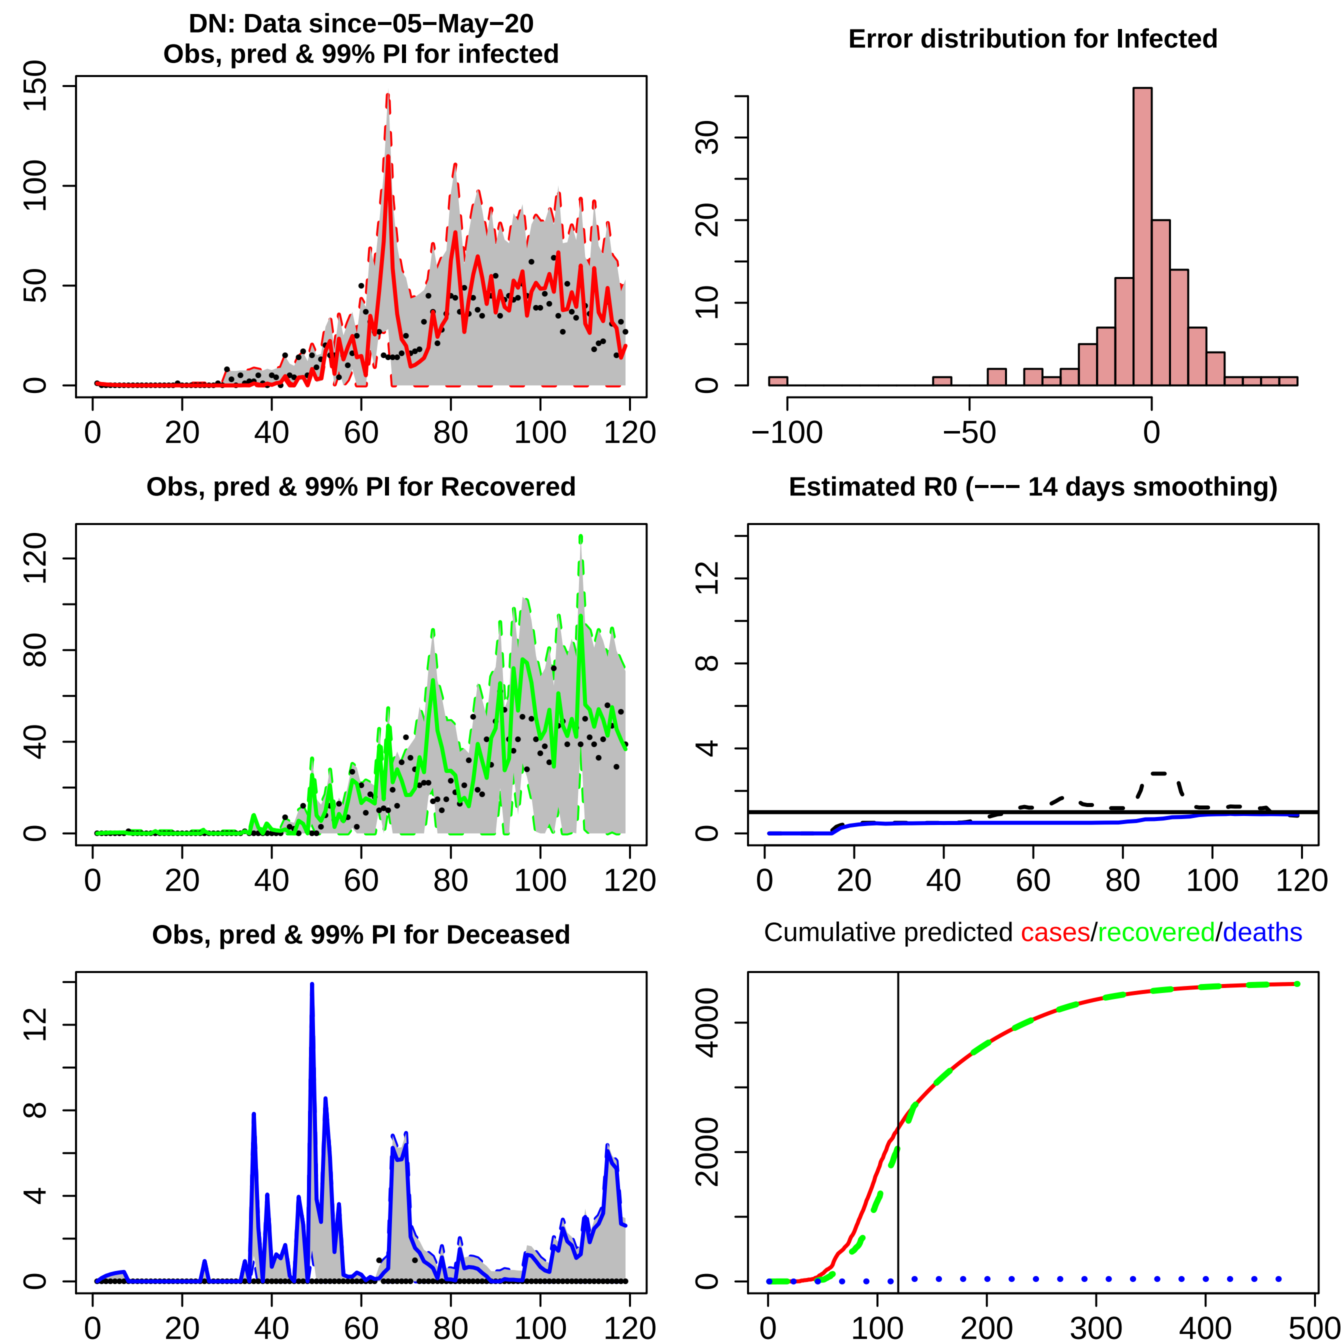
DN: Data since−05−May−20
Obs, pred & 99% PI for infected
0 50 100 150
0 20 40 60 80 100 120
Error distribution for Infected
0 10 20 30
−100 −50 0
Obs, pred & 99% PI for Recovered
0 40 80 120
0 20 40 60 80 100 120
Estimated R0 (−−− 14 days smoothing)
0 4 8 12
0 20 40 60 80 100 120
Obs, pred & 99% PI for Deceased
0 4 8 12
0 20 40 60 80 100 120
Cumulative predicted cases/recovered/deaths
0 2000 4000
0 100 200 300 400 500

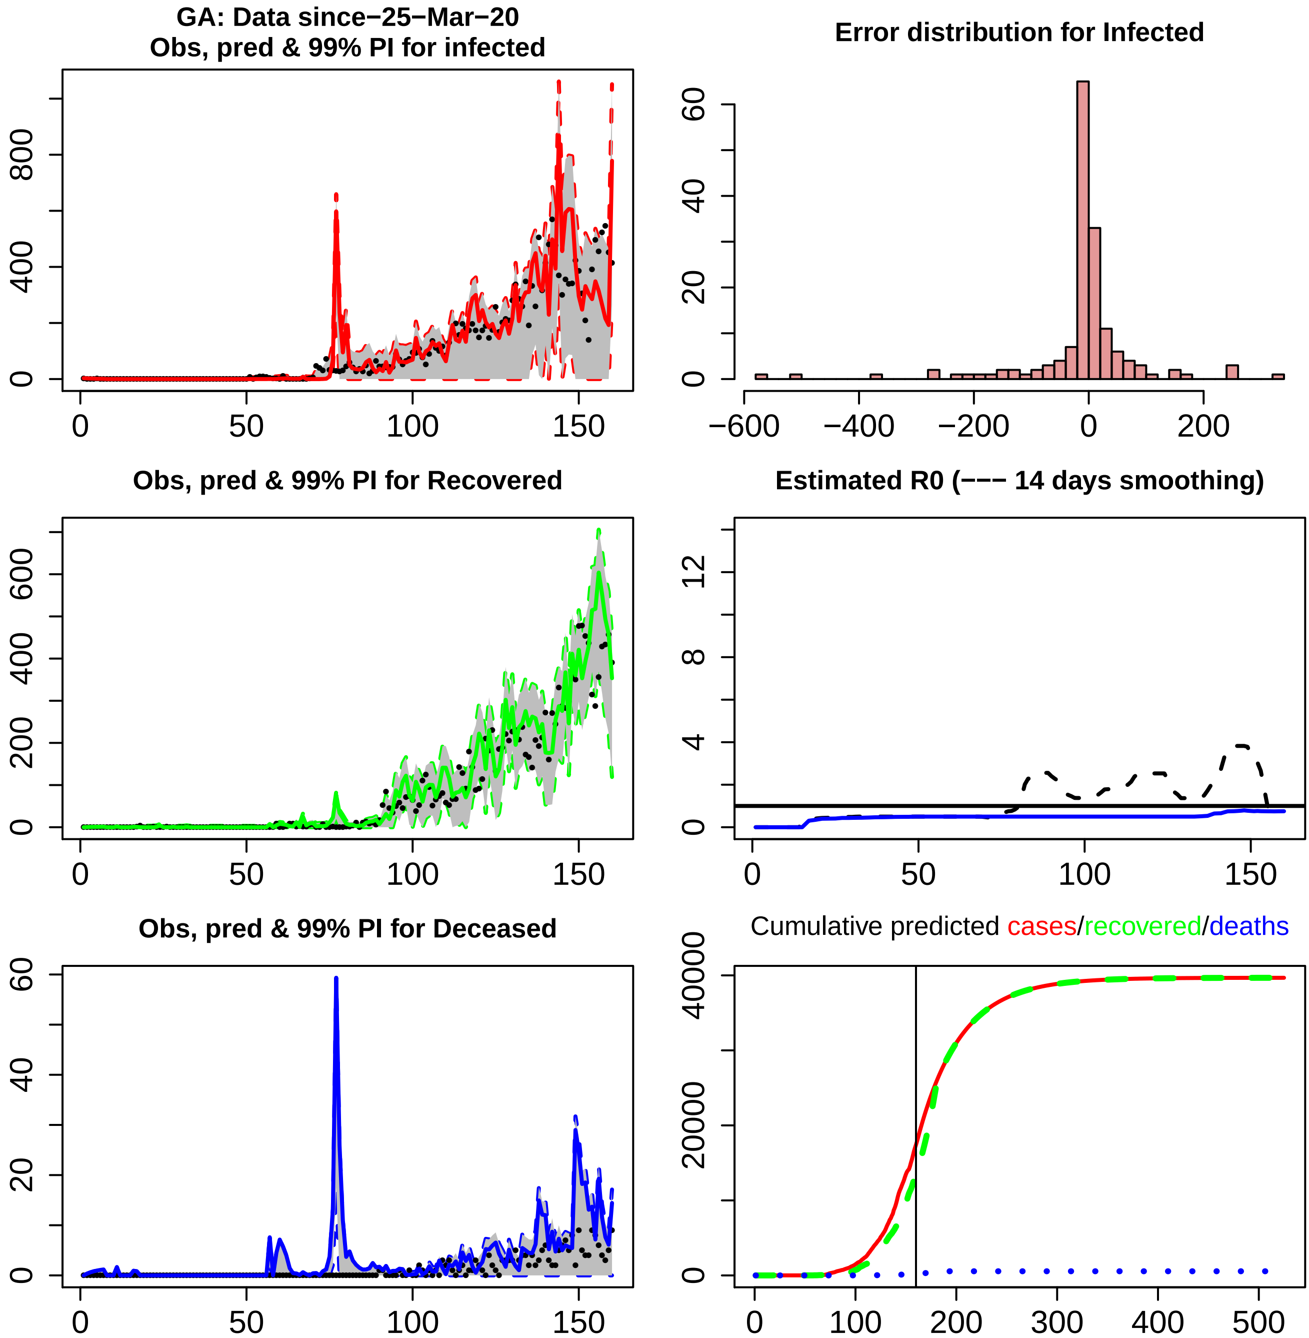
GA: Data since−25−Mar−20
Obs, pred & 99% PI for infected
0
400
800
0
50
100
150
Error distribution for Infected
0
20
40
60
−600
−400
−200
0
200
Obs, pred & 99% PI for Recovered
0
200
400
600
0
50
100
150
Estimated R0 (−−− 14 days smoothing)
0
4
8
12
0
50
100
150
Obs, pred & 99% PI for Deceased
0
20
40
60
0
50
100
150
Cumulative predicted cases/recovered/deaths
0
20000
40000
0
100
200
300
400
500

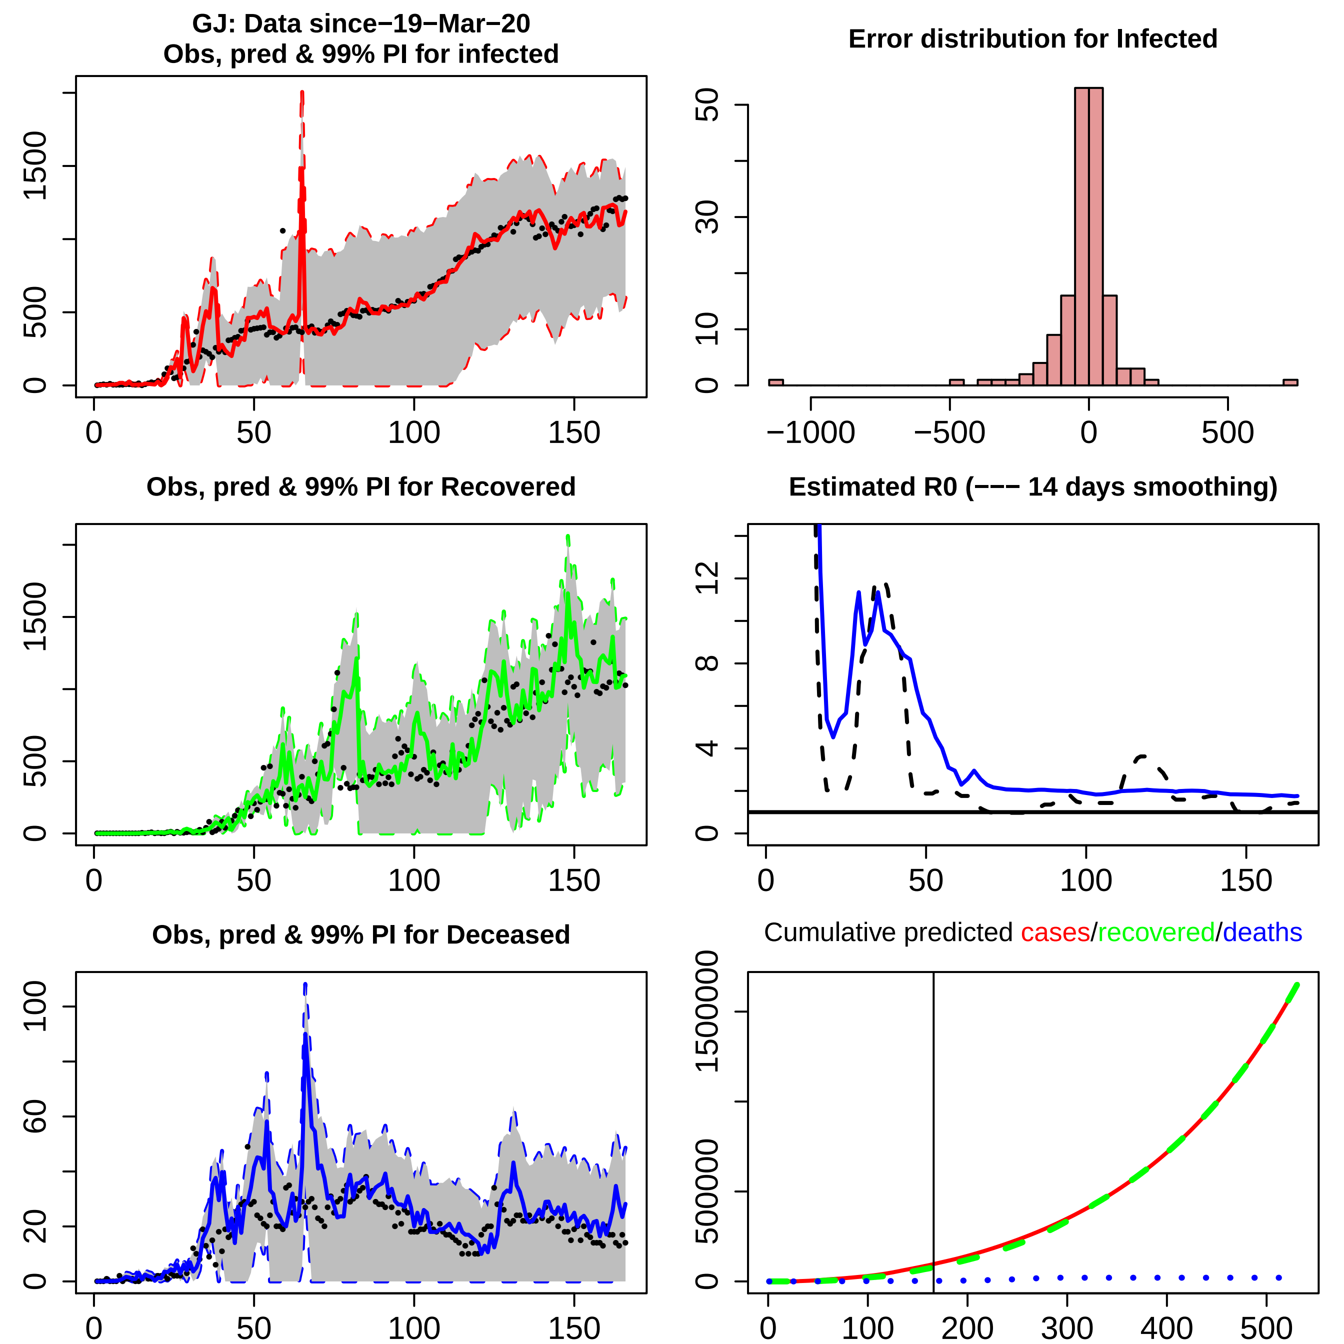

GJ: Data since−19−Mar−20
Obs, pred & 99% PI for infected
Error distribution for Infected
Obs, pred & 99% PI for Recovered
Estimated R0 (−−− 14 days smoothing)
Obs, pred & 99% PI for Deceased
Cumulative predicted cases/recovered/deaths

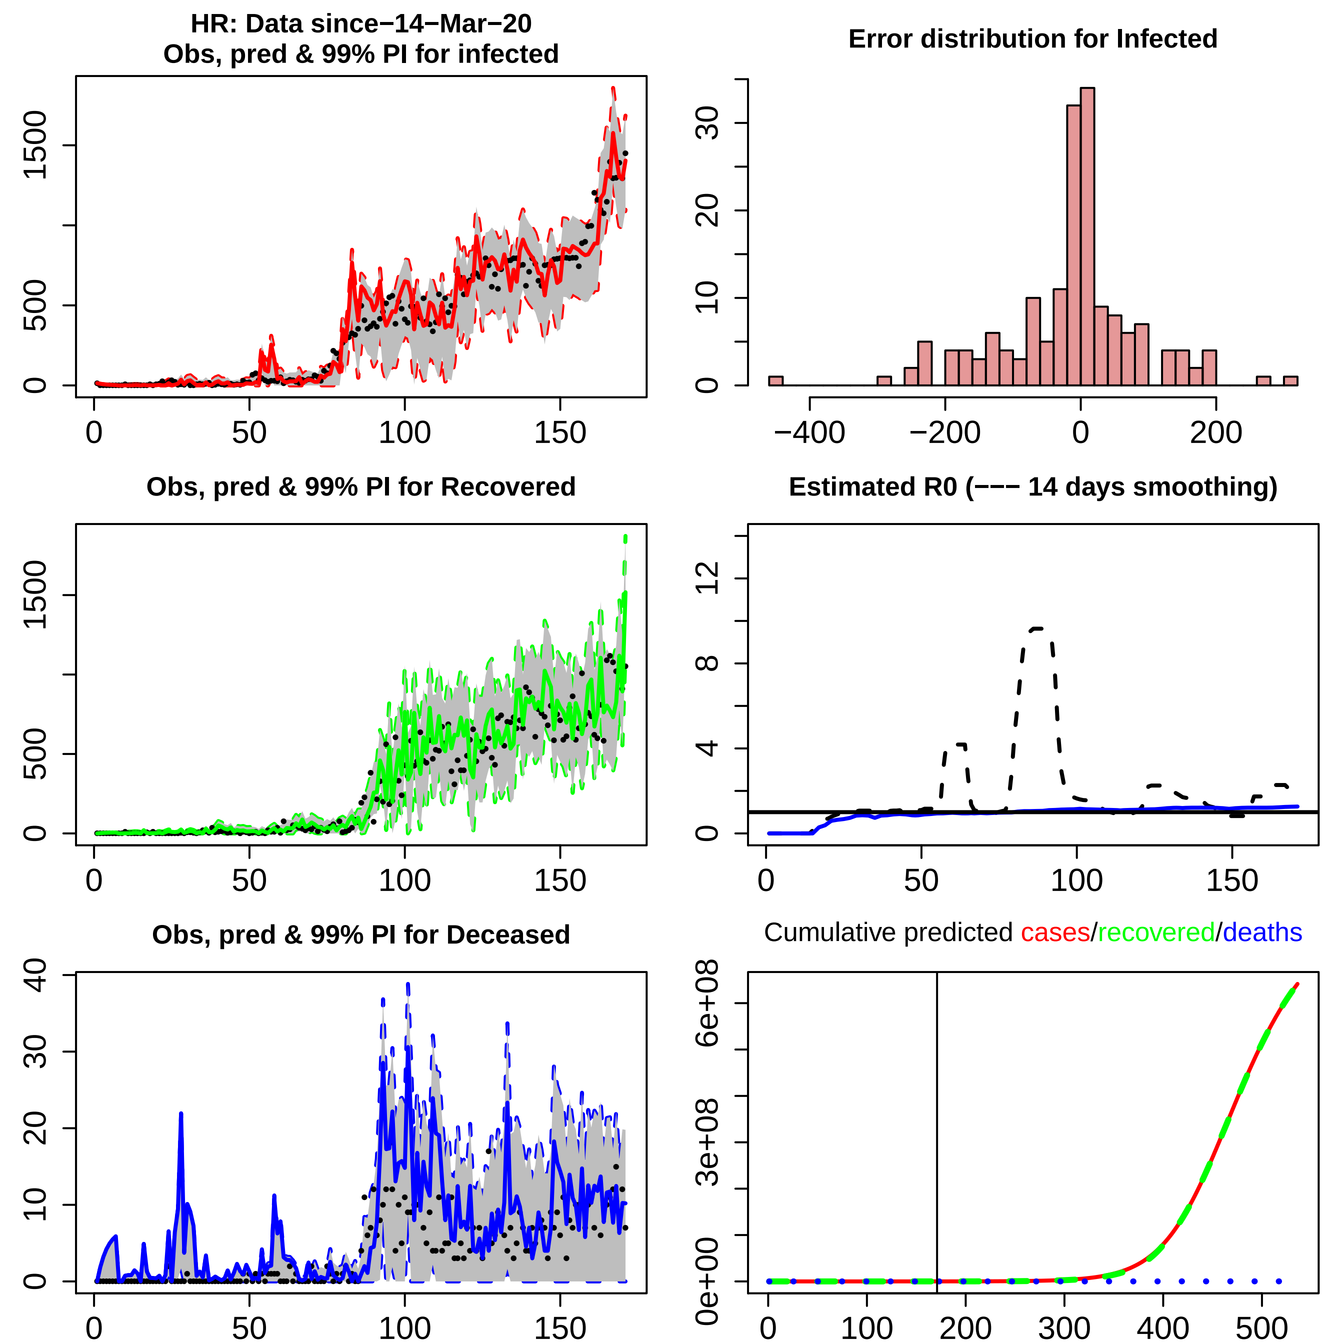
HR: Data since−14−Mar−20
Obs, pred & 99% PI for infected
Error distribution for Infected
Obs, pred & 99% PI for Recovered
Estimated R0 (−−− 14 days smoothing)
Obs, pred & 99% PI for Deceased
Cumulative predicted cases/recovered/deaths

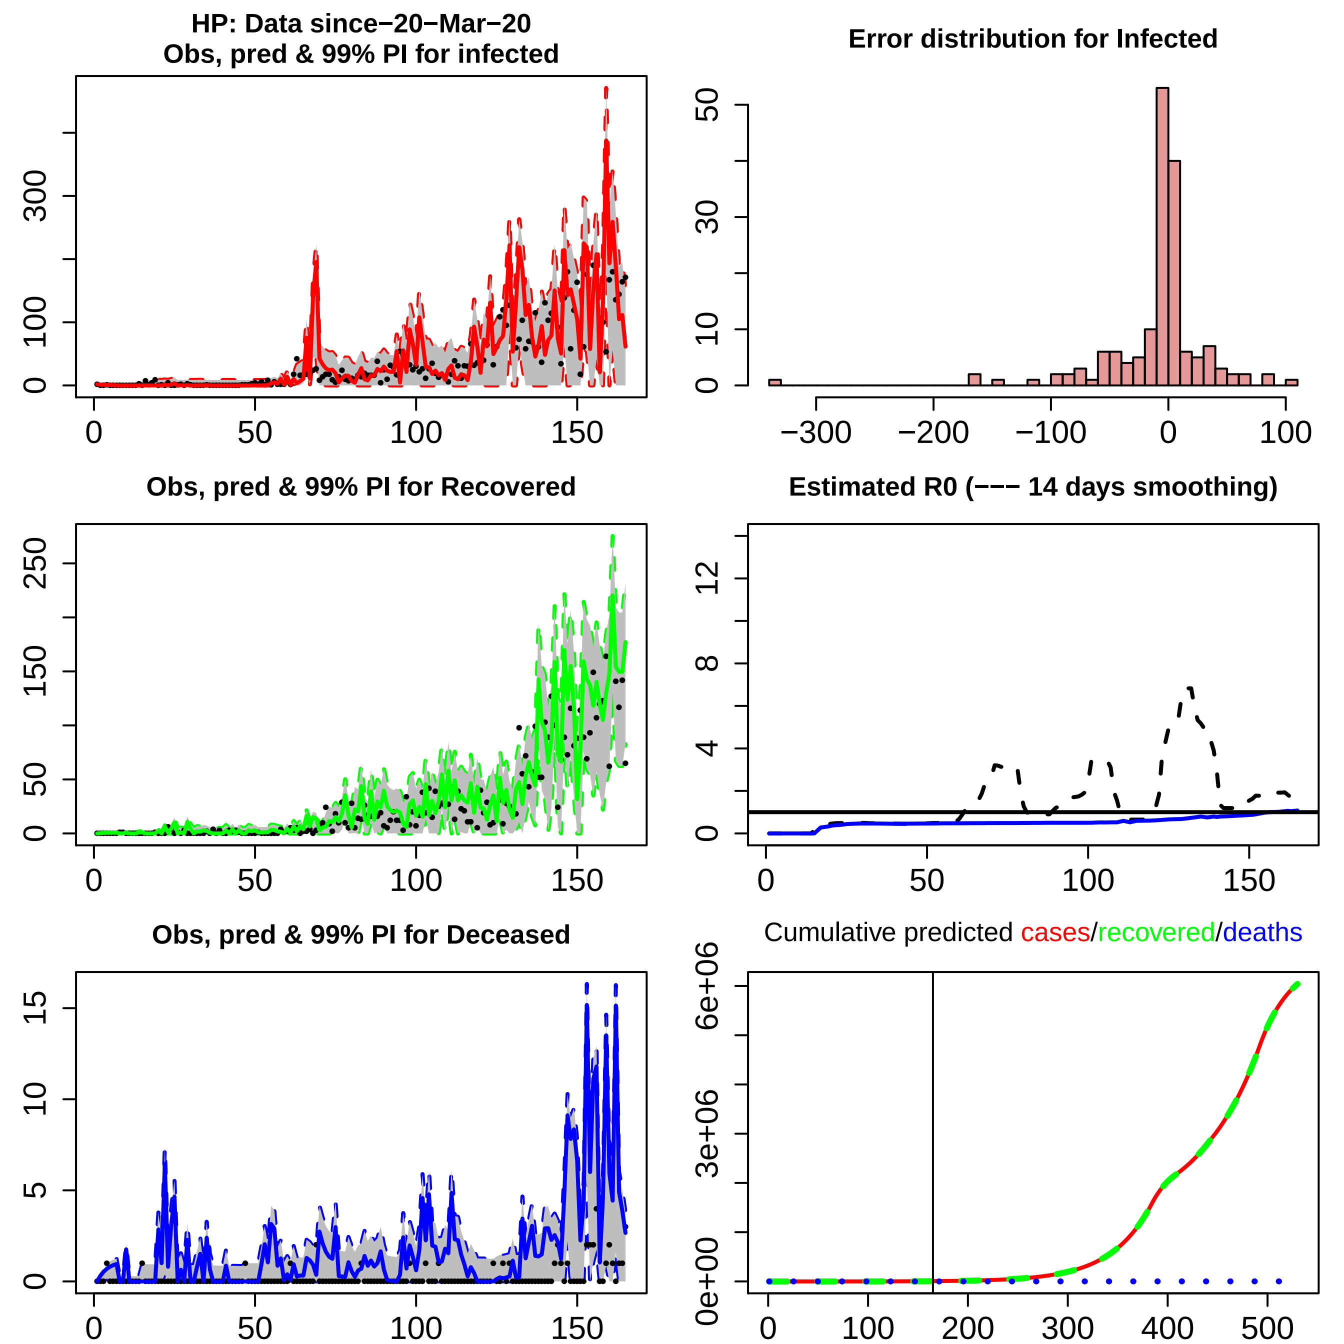
HP: Data since−20−Mar−20
Obs, pred & 99% PI for infected
Error distribution for Infected
Obs, pred & 99% PI for Recovered
Estimated R0 (−−− 14 days smoothing)
Obs, pred & 99% PI for Deceased
Cumulative predicted cases/recovered/deaths

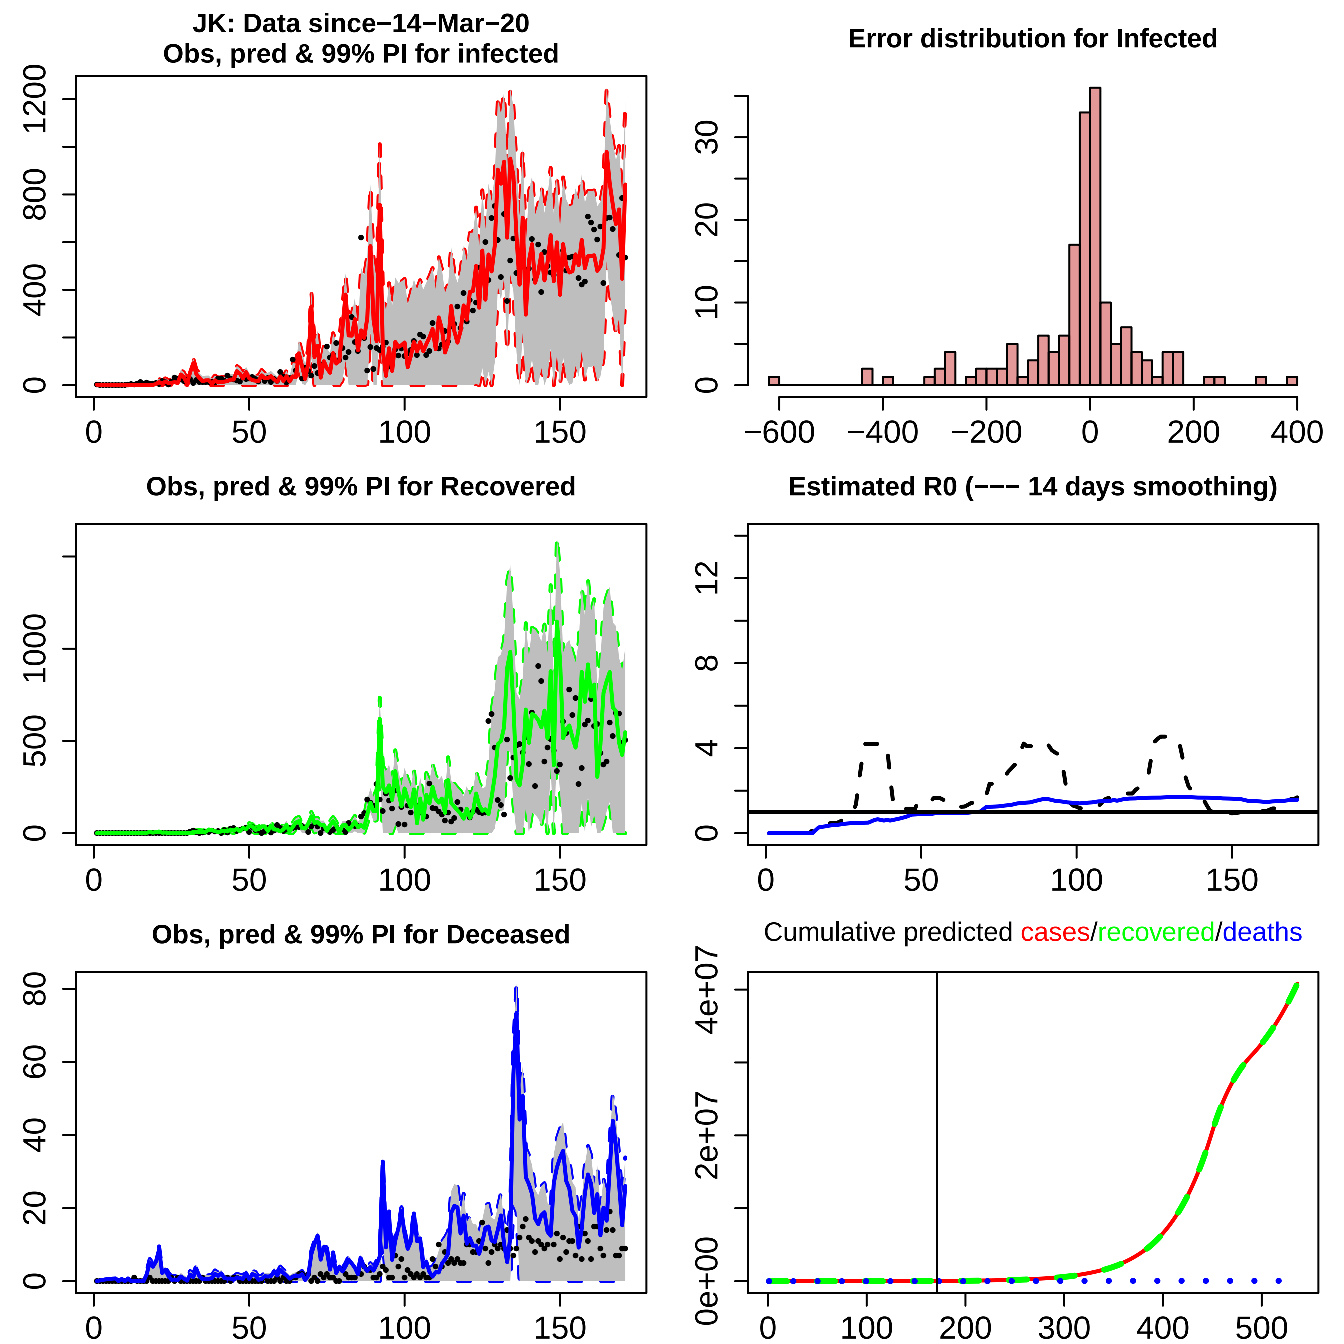
JK: Data since−14−Mar−20
Obs, pred & 99% PI for infected
0 400 800 1200
0 50 100 150
Error distribution for Infected
0 10 20 30
−600 −400 −200 0 200 400
Obs, pred & 99% PI for Recovered
0 500 1000
0 50 100 150
Estimated R0 (−−− 14 days smoothing)
0 4 8 12
0 50 100 150
Obs, pred & 99% PI for Deceased
0 20 40 60 80
0 50 100 150
Cumulative predicted cases/recovered/deaths
0e+00 2e+07 4e+07
0 100 200 300 400 500

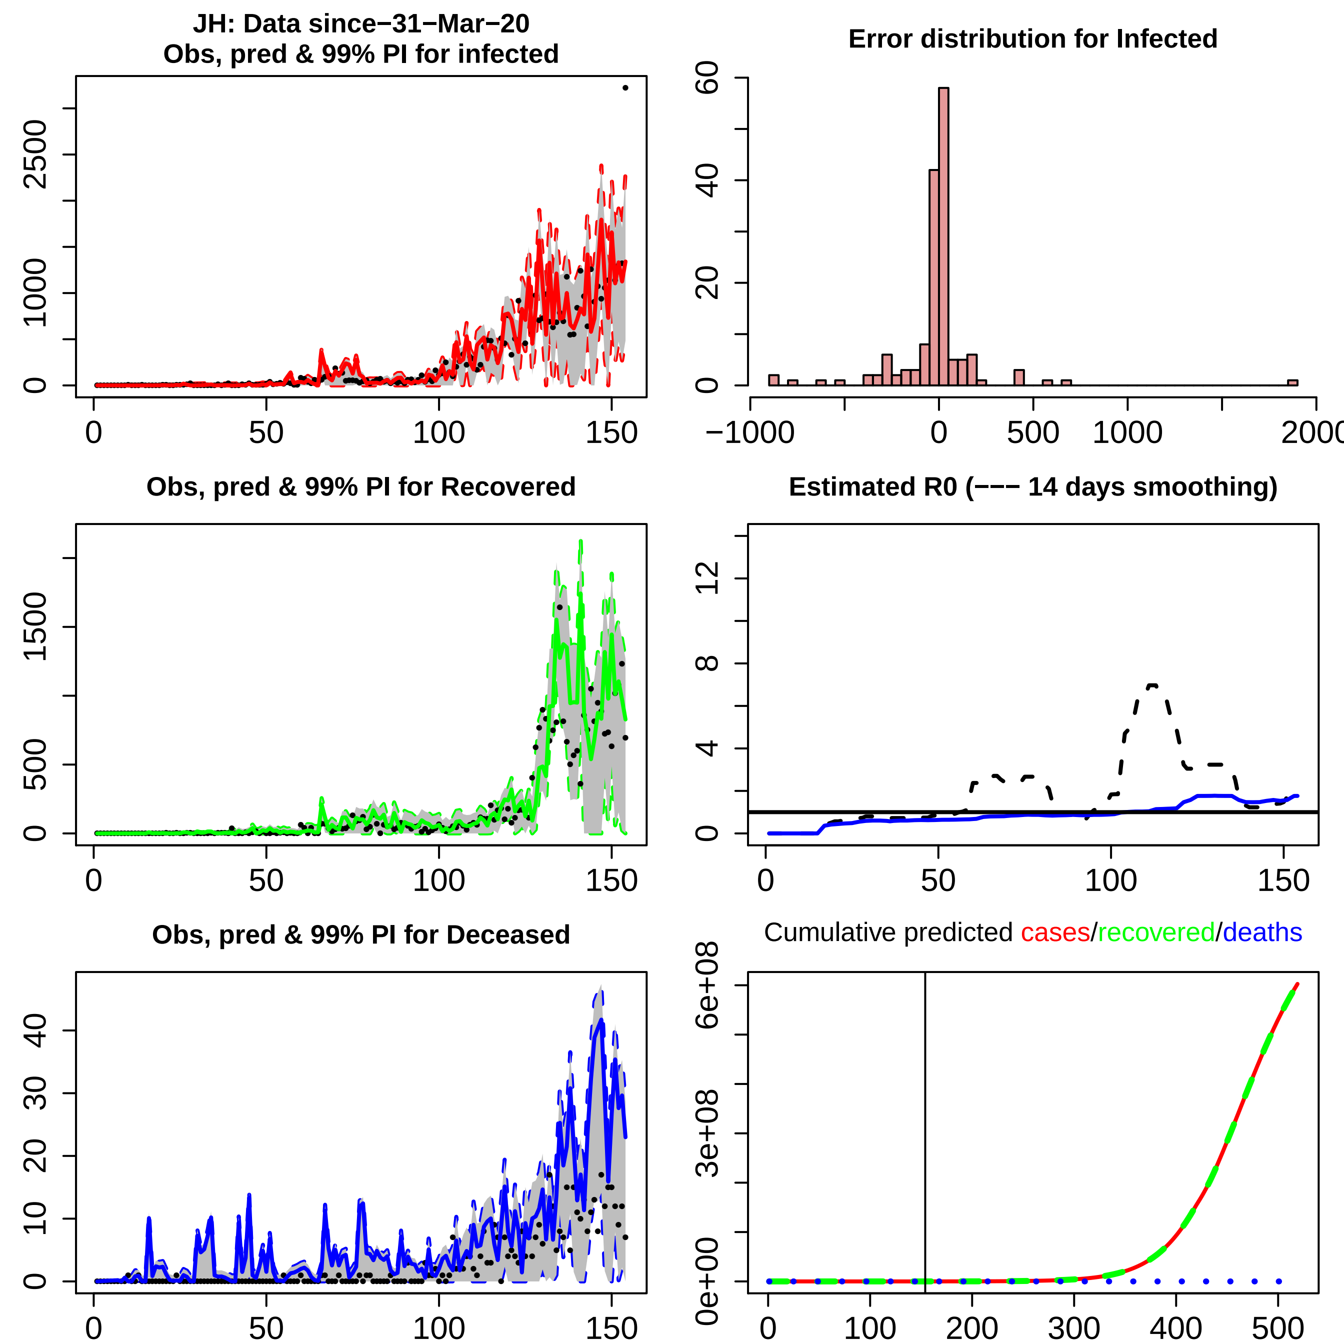
JH: Data since−31−Mar−20
Obs, pred & 99% PI for infected
Error distribution for Infected
Obs, pred & 99% PI for Recovered
Estimated R0 (−−− 14 days smoothing)
Obs, pred & 99% PI for Deceased
Cumulative predicted cases/recovered/deaths

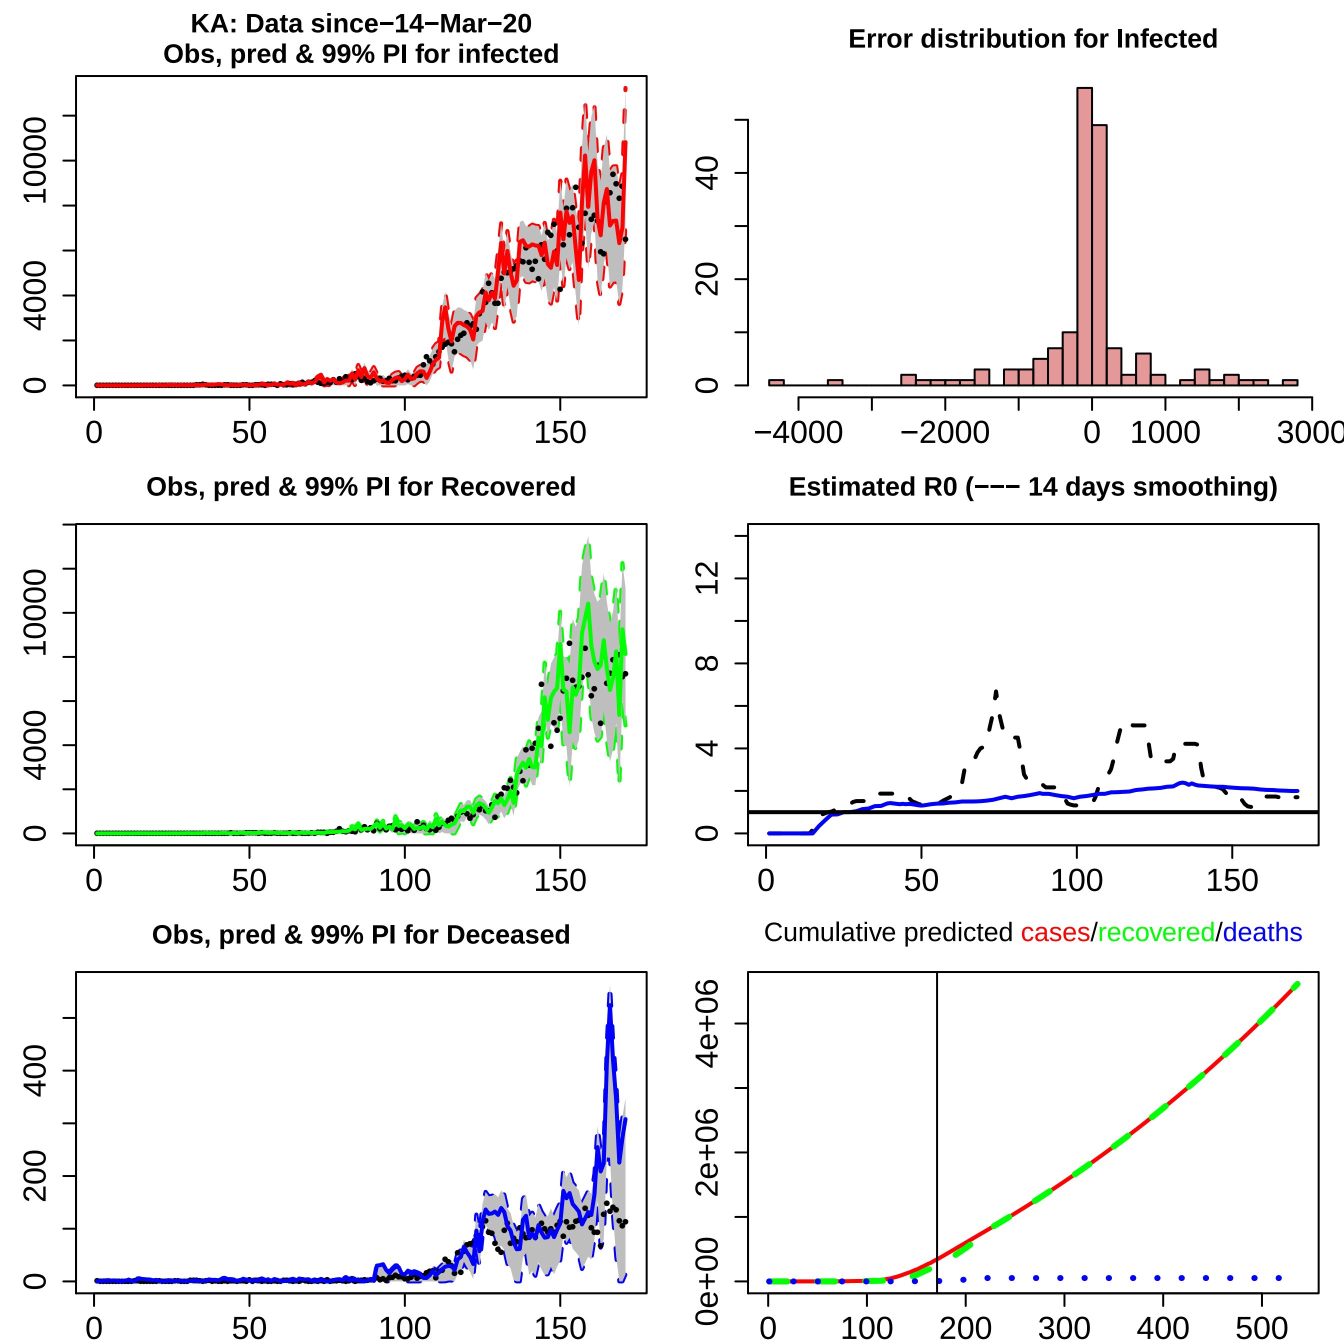
KA: Data since−14−Mar−20
Obs, pred & 99% PI for infected
Error distribution for Infected
Obs, pred & 99% PI for Recovered
Estimated R0 (−−− 14 days smoothing)
Obs, pred & 99% PI for Deceased
Cumulative predicted cases/recovered/deaths

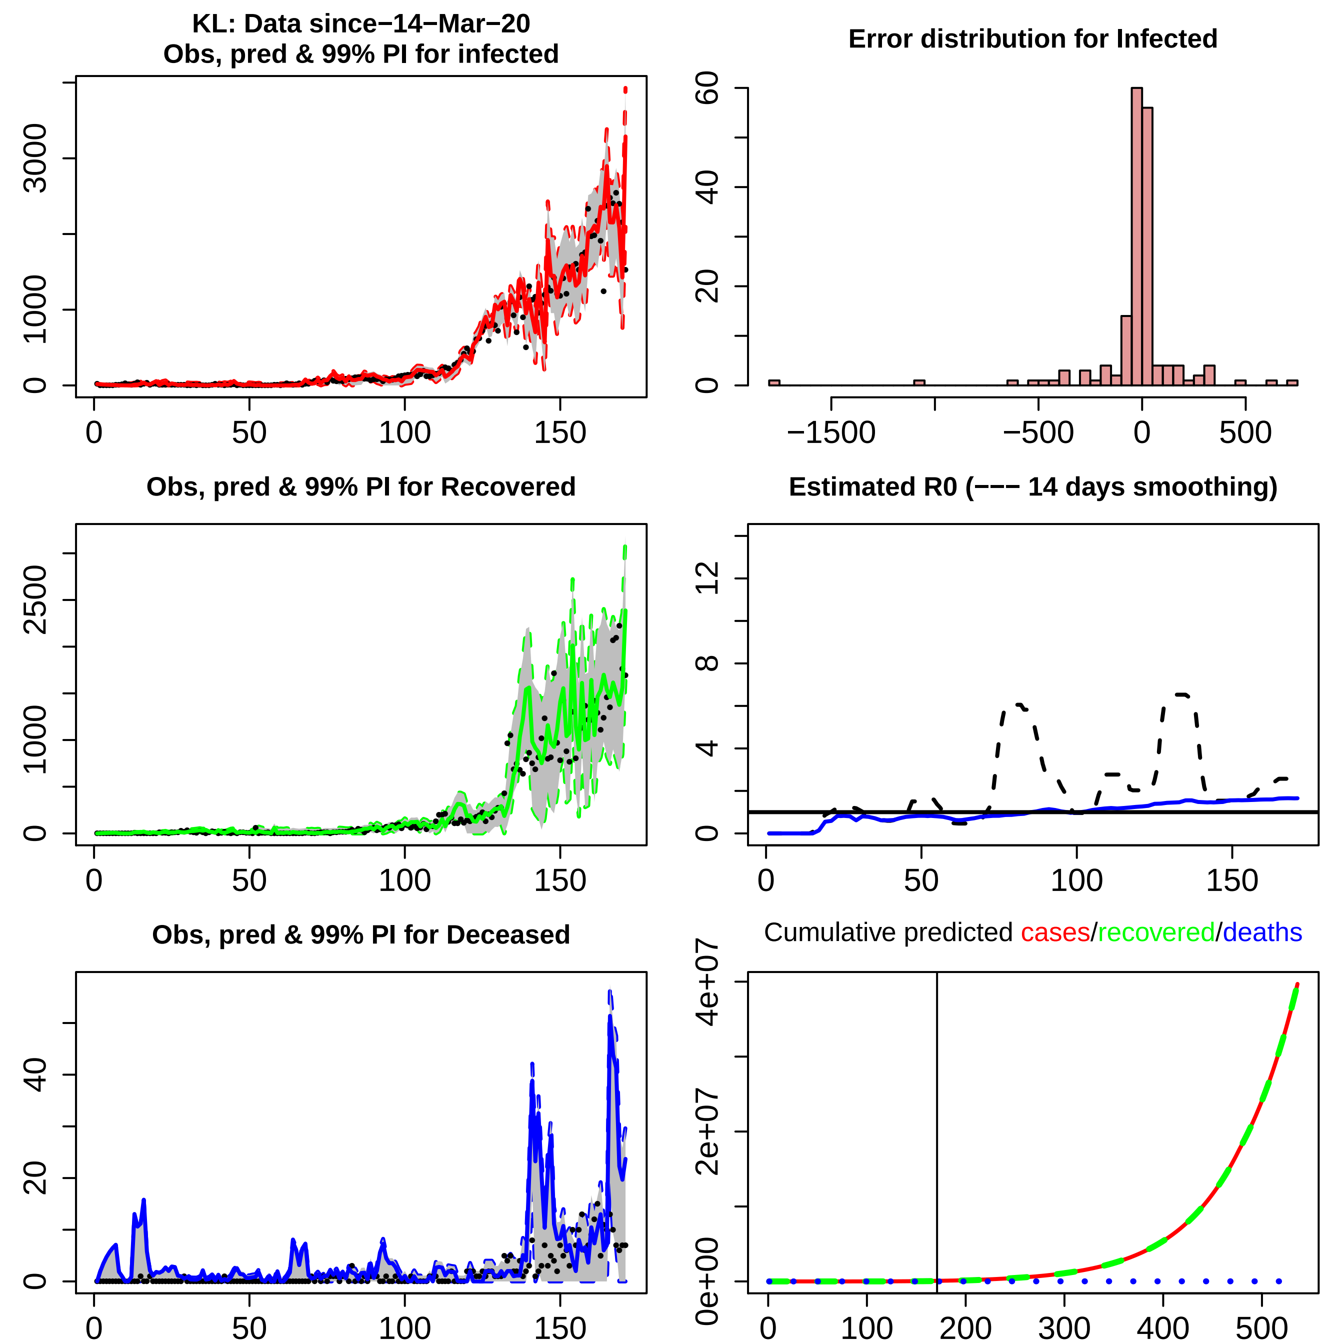

KL: Data since−14−Mar−20
Obs, pred & 99% PI for infected
Error distribution for Infected
Obs, pred & 99% PI for Recovered
Estimated R0 (−−− 14 days smoothing)
Obs, pred & 99% PI for Deceased
Cumulative predicted cases/recovered/deaths

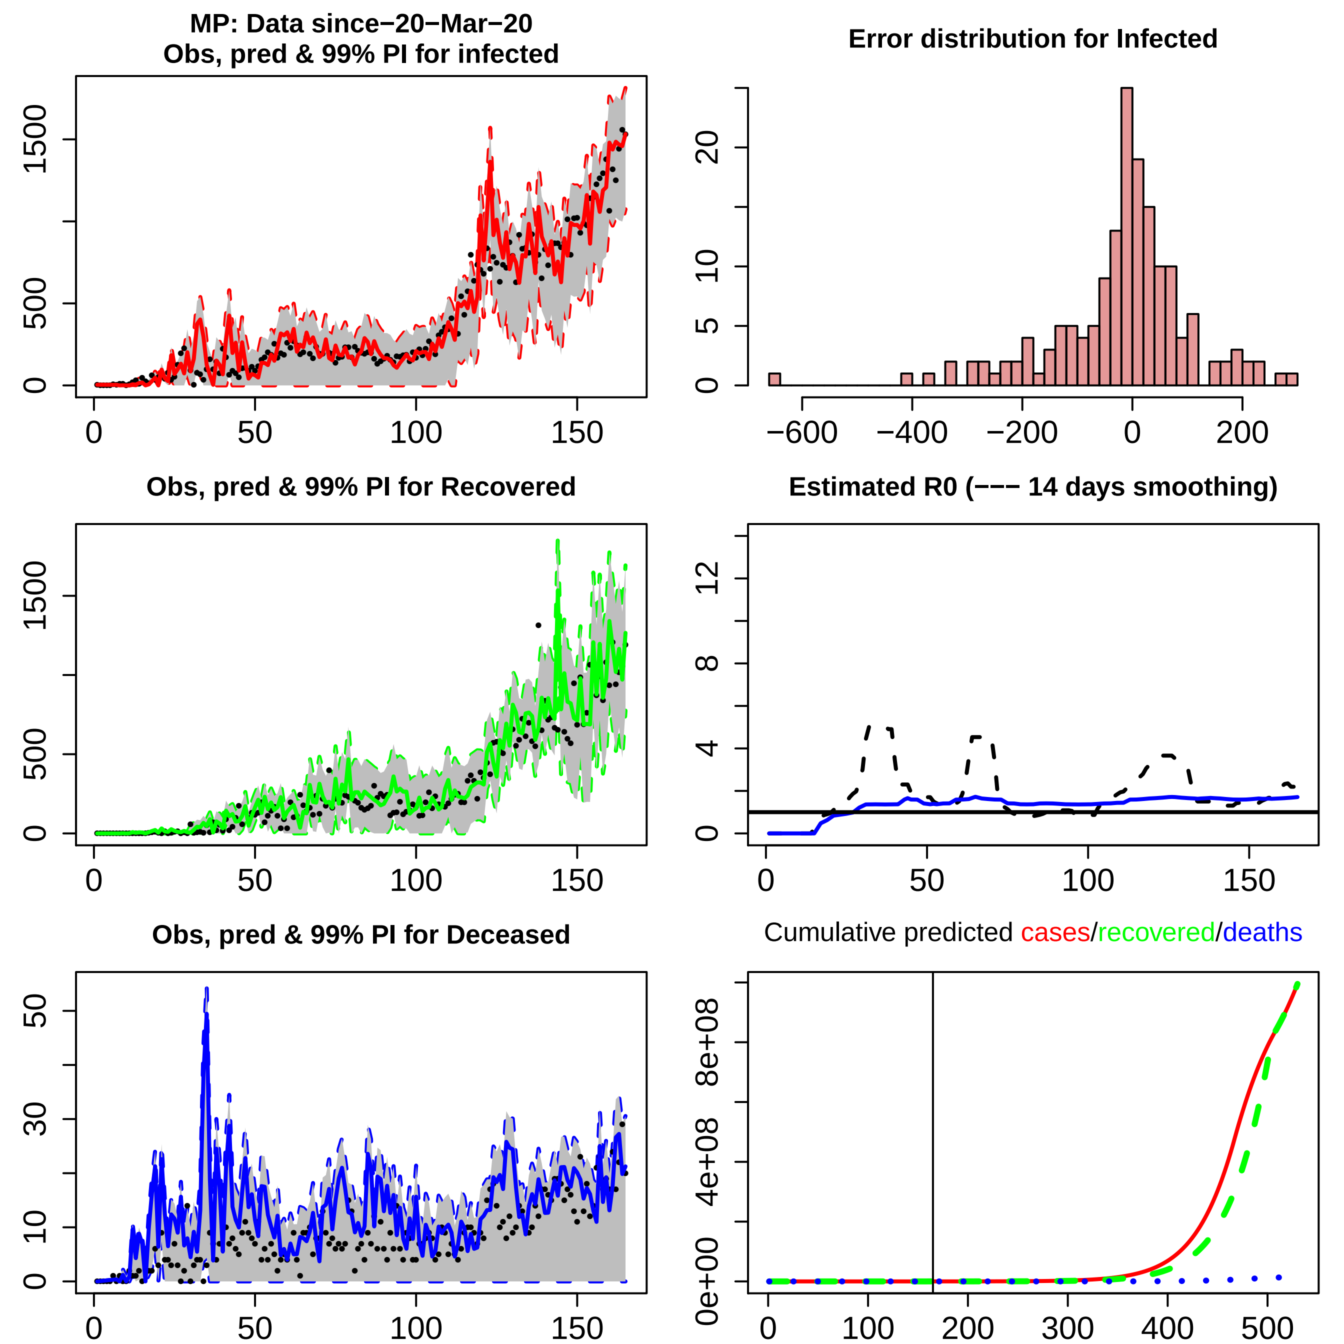
MP: Data since−20−Mar−20
Obs, pred & 99% PI for infected
Error distribution for Infected
Obs, pred & 99% PI for Recovered
Estimated R0 (−−− 14 days smoothing)
Obs, pred & 99% PI for Deceased
Cumulative predicted cases/recovered/deaths

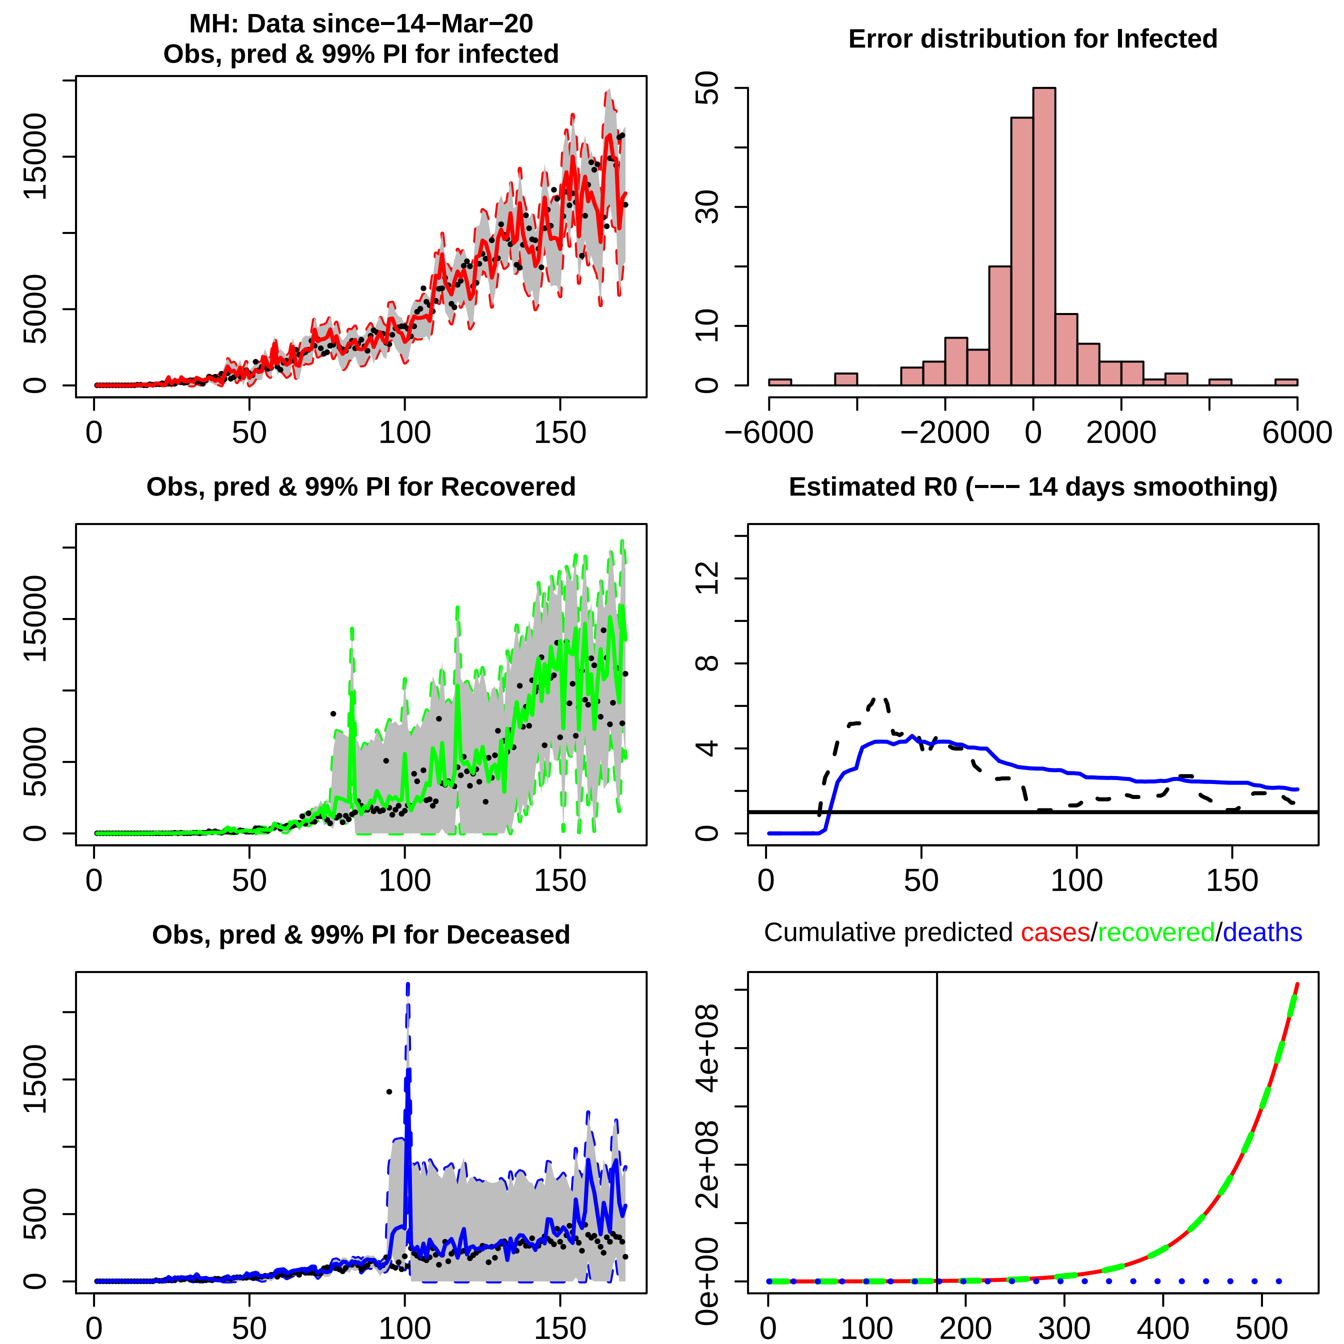
MH: Data since−14−Mar−20
Obs, pred & 99% PI for infected
0
5000
15000
0
50
100
150
Error distribution for Infected
0
10
30
50
−6000
−2000
0
2000
6000
Obs, pred & 99% PI for Recovered
0
5000
15000
0
50
100
150
Estimated R0 (−−− 14 days smoothing)
0
4
8
12
0
50
100
150
Obs, pred & 99% PI for Deceased
0
500
1500
0
50
100
150
Cumulative predicted cases/recovered/deaths
0e+00
2e+08
4e+08
0
100
200
300
400
500

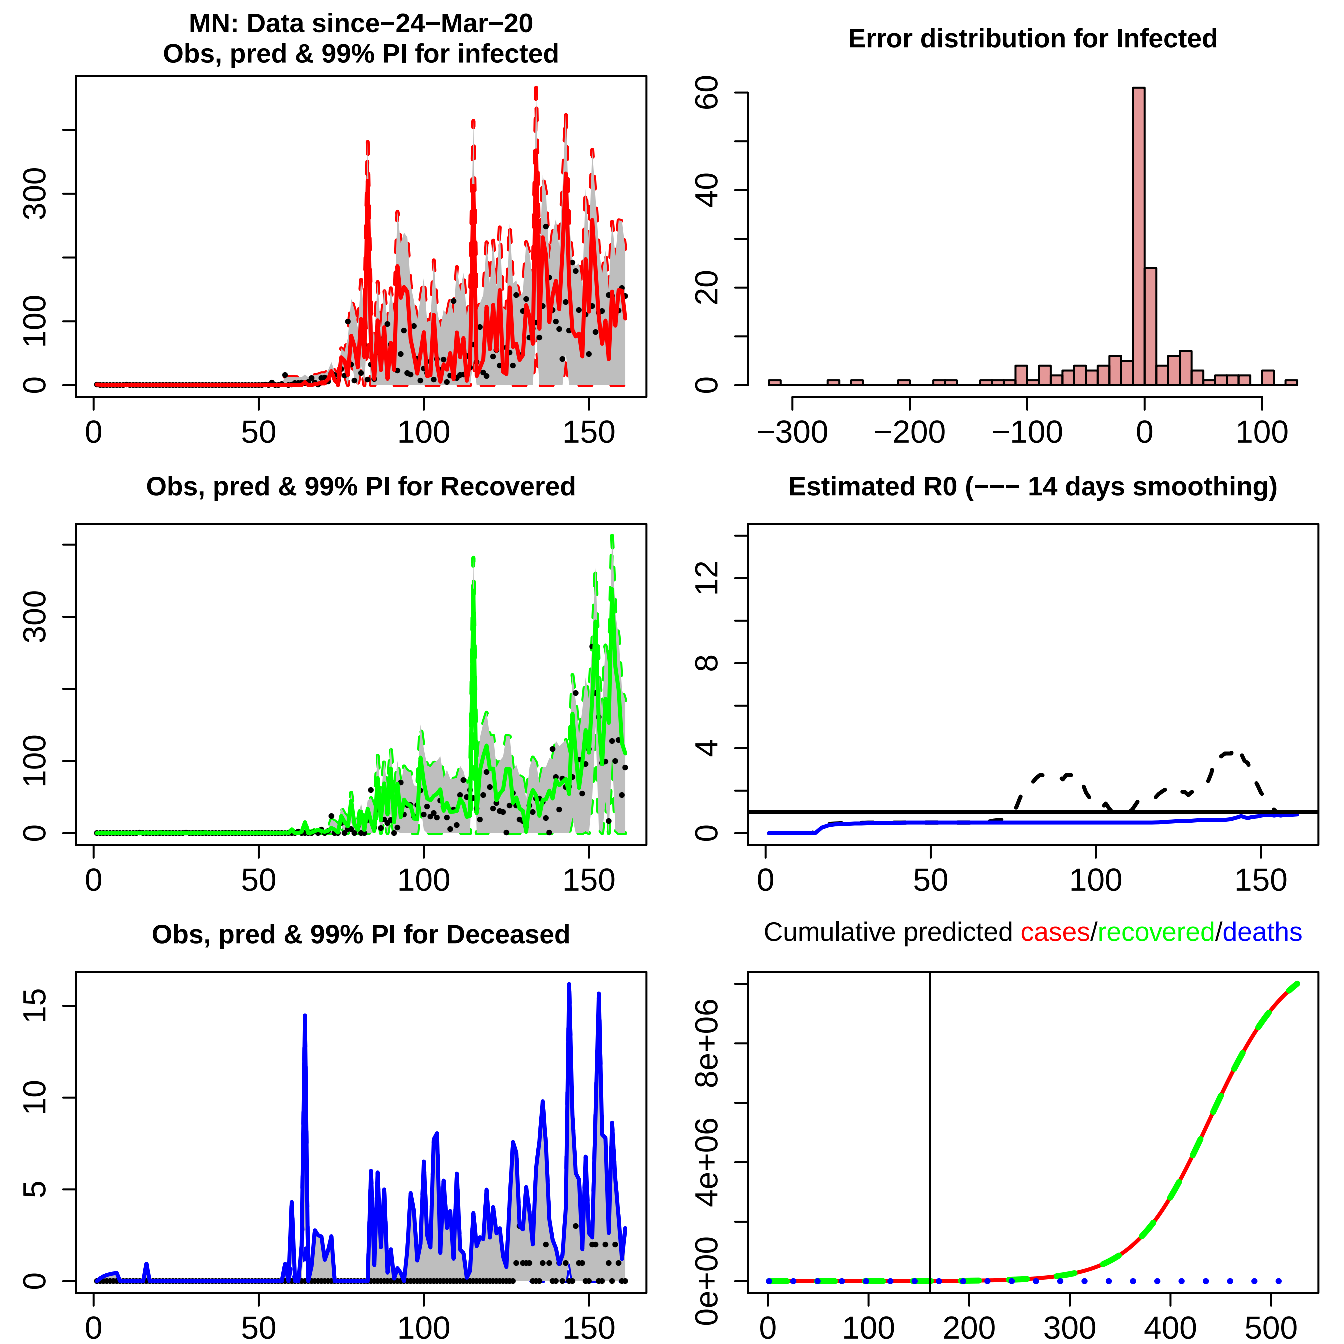

MN: Data since−24−Mar−20
Obs, pred & 99% PI for infected
Error distribution for Infected
Obs, pred & 99% PI for Recovered
Estimated R0 (−−− 14 days smoothing)
Obs, pred & 99% PI for Deceased
Cumulative predicted cases/recovered/deaths

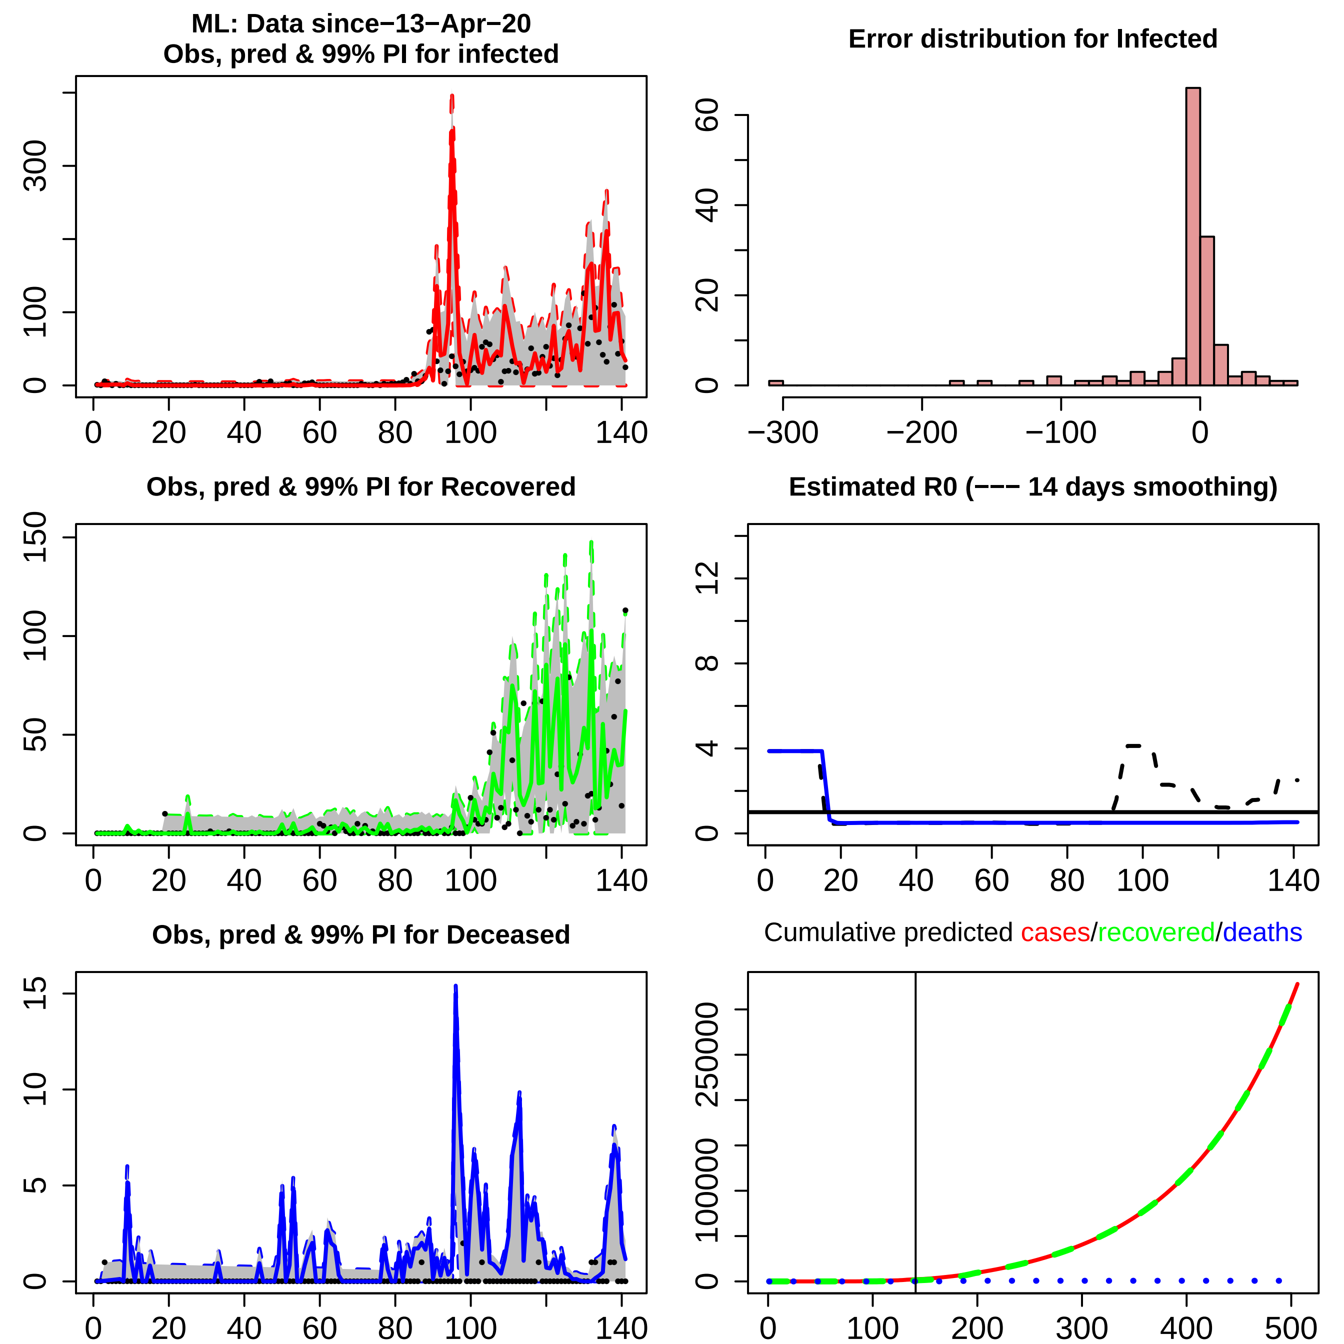
ML: Data since−13−Apr−20
Obs, pred & 99% PI for infected
0
100
300
0
20
40
60
80
100
140
Error distribution for Infected
0
20
40
60
−300
−200
−100
0
Obs, pred & 99% PI for Recovered
0
50
100
150
0
20
40
60
80
100
140
Estimated R0 (−−− 14 days smoothing)
0
4
8
12
0
20
40
60
80
100
140
Obs, pred & 99% PI for Deceased
0
5
10
15
0
20
40
60
80
100
140
Cumulative predicted cases/recovered/deaths
0
100000
250000
0
100
200
300
400
500

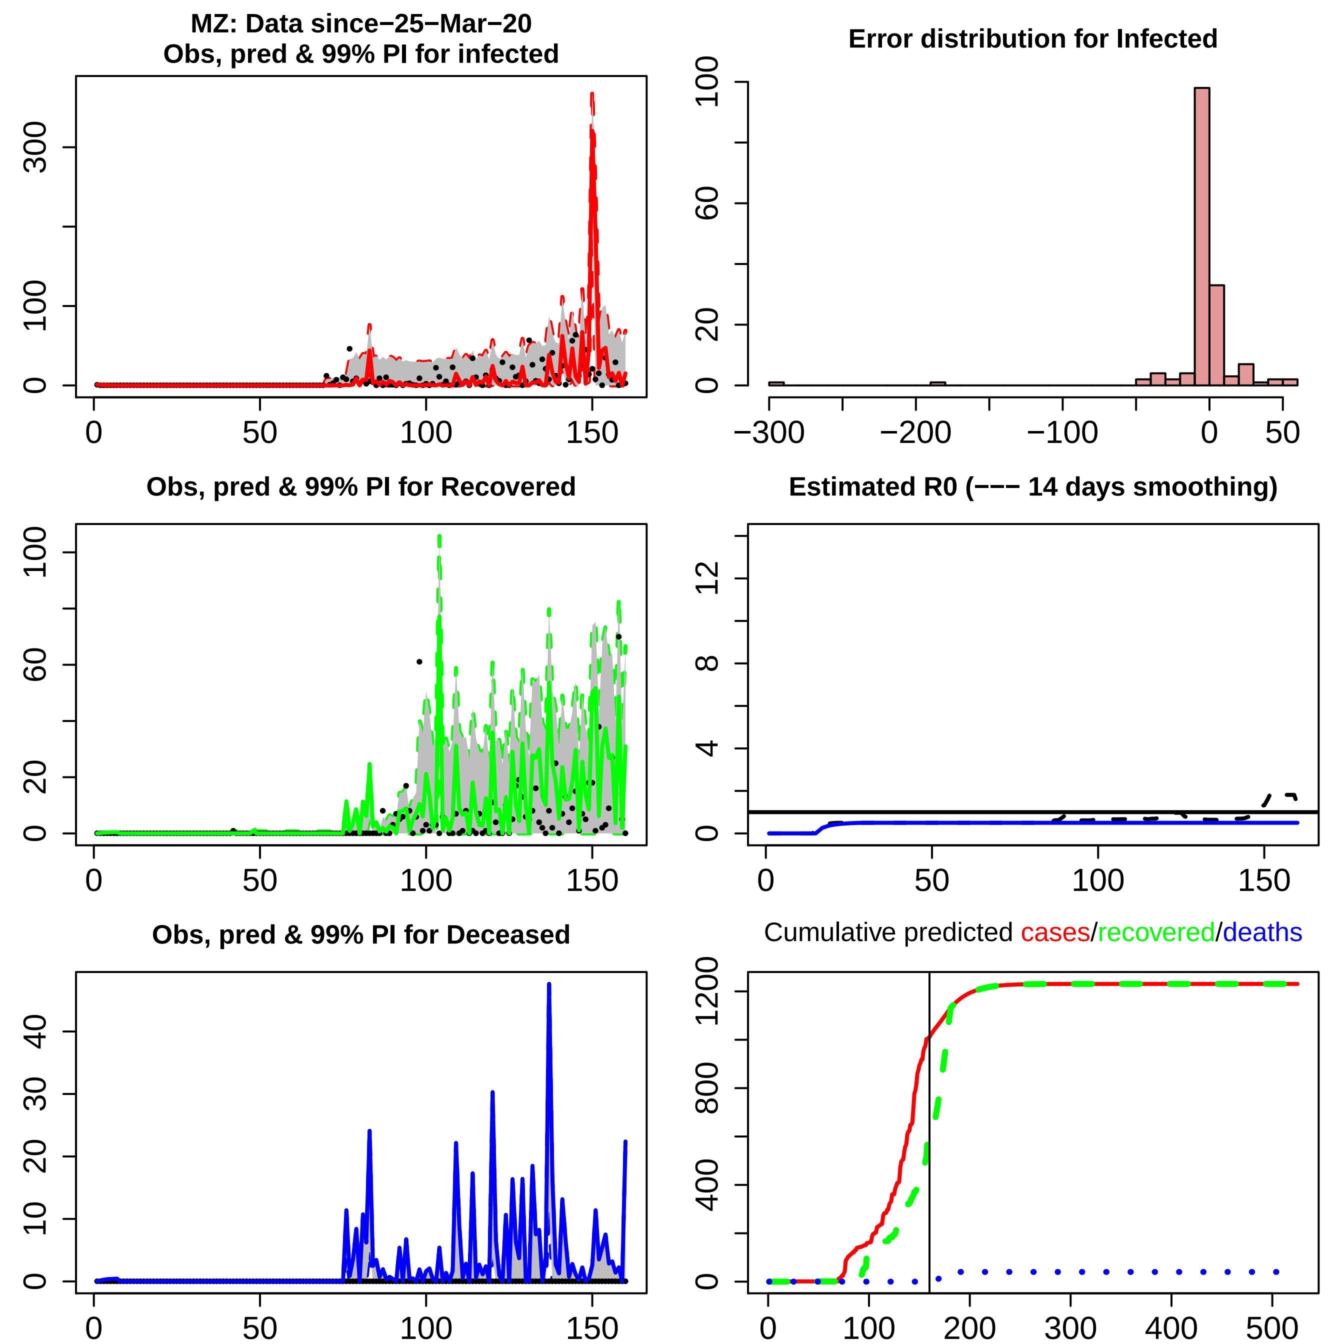
MZ: Data since−25−Mar−20
Obs, pred & 99% PI for infected
0
100
300
0
50
100
150
Error distribution for Infected
0
20
60
100
−300
−200
−100
0
50
Obs, pred & 99% PI for Recovered
0
20
60
100
0
50
100
150
Estimated R0 (−−− 14 days smoothing)
0
4
8
12
0
50
100
150
Obs, pred & 99% PI for Deceased
0
10
20
30
40
0
50
100
150
Cumulative predicted cases/recovered/deaths
0
400
800
1200
0
100
200
300
400
500

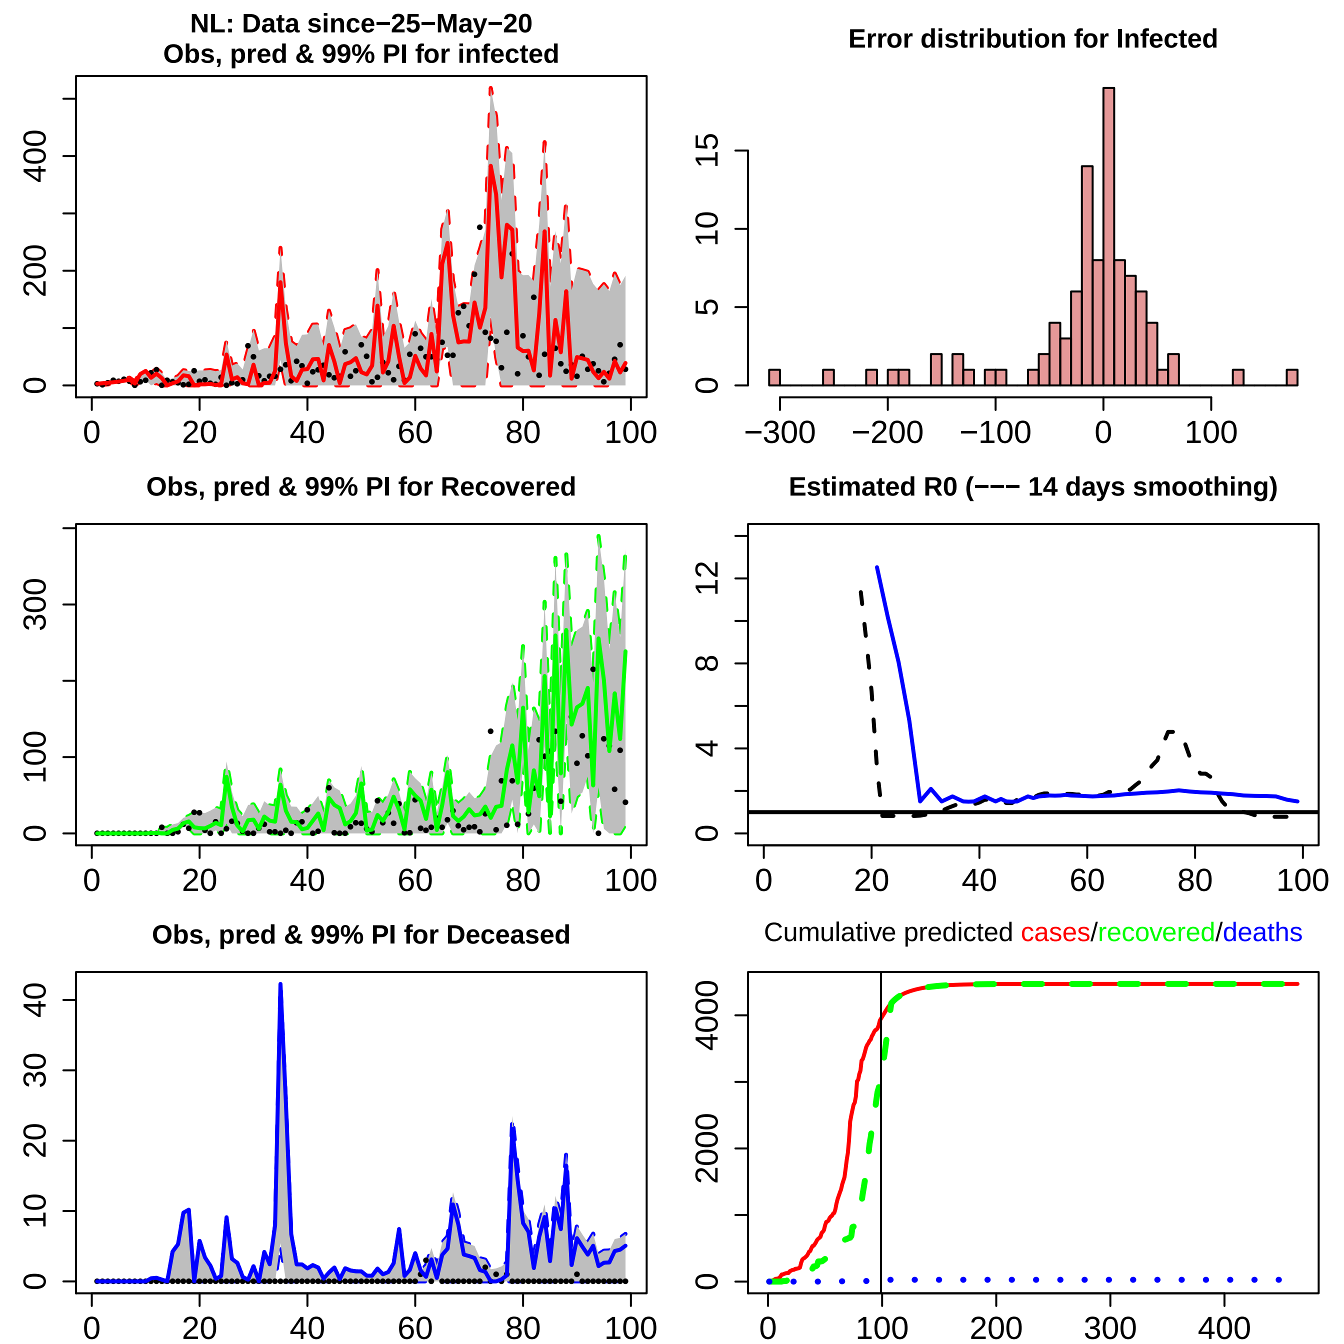
NL: Data since−25−May−20
Obs, pred & 99% PI for infected
Error distribution for Infected
Obs, pred & 99% PI for Recovered
Estimated R0 (−−− 14 days smoothing)
Obs, pred & 99% PI for Deceased
Cumulative predicted cases/recovered/deaths

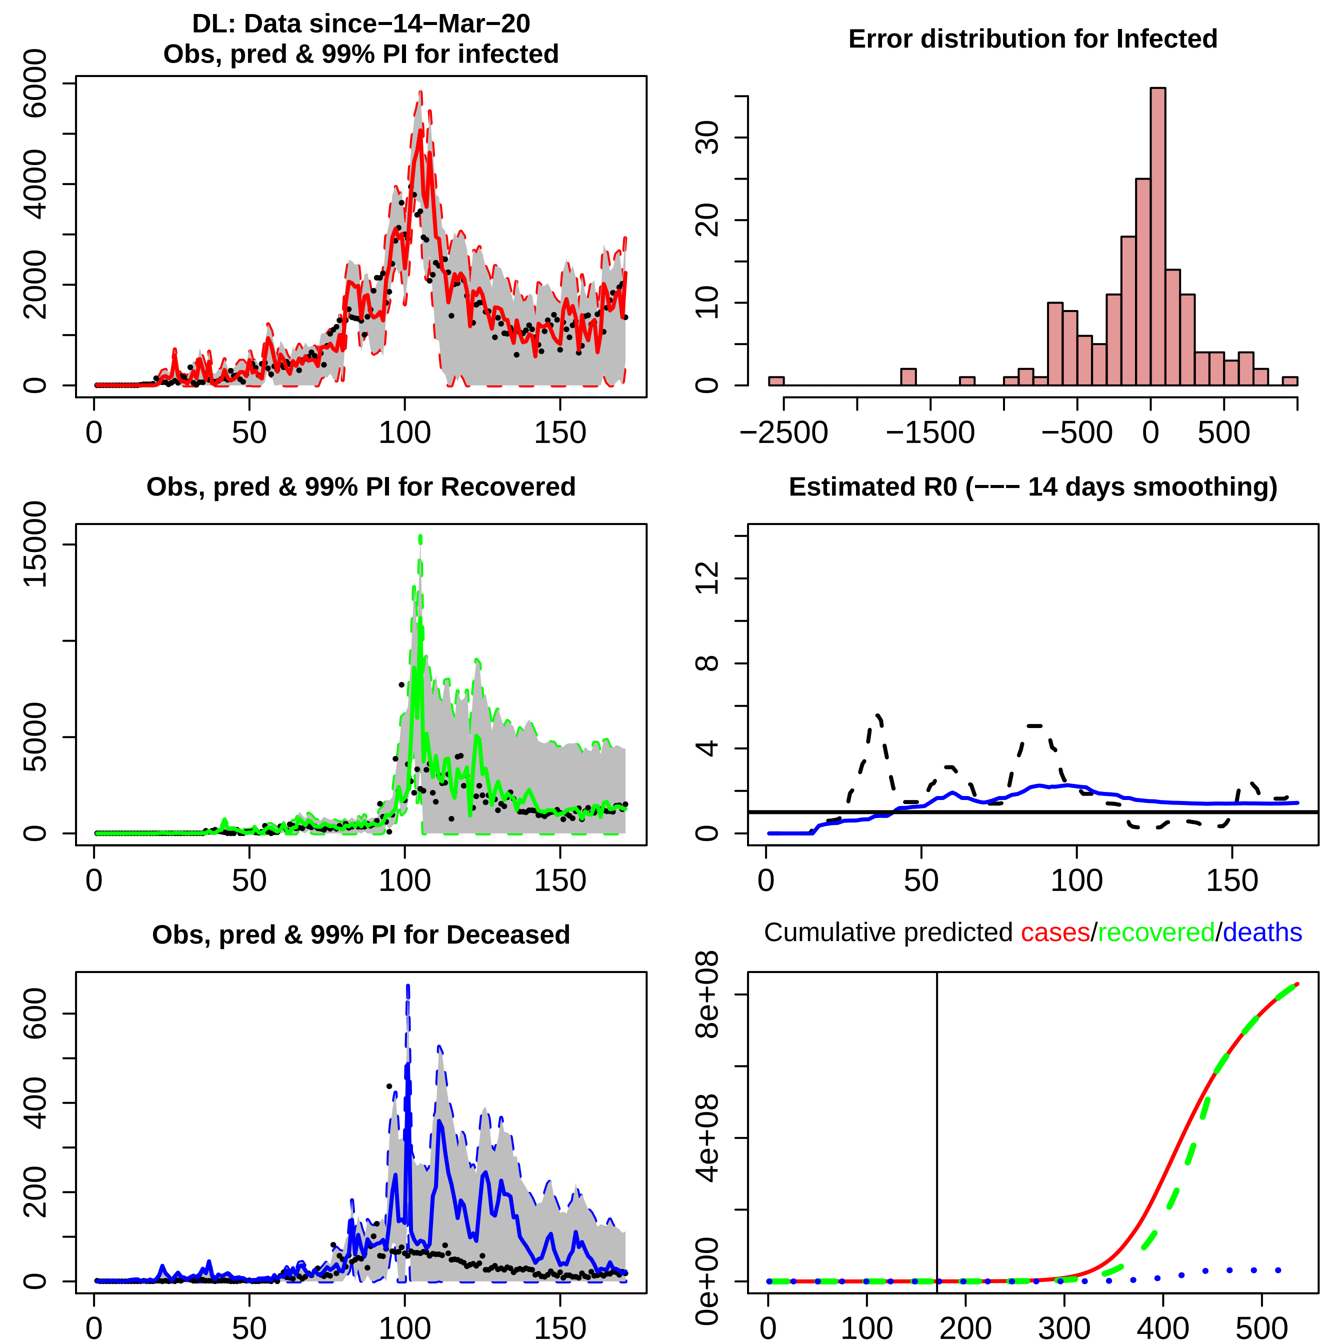

DL: Data since−14−Mar−20
Obs, pred & 99% PI for infected
Error distribution for Infected
Obs, pred & 99% PI for Recovered
Estimated R0 (−−− 14 days smoothing)
Obs, pred & 99% PI for Deceased
Cumulative predicted cases/recovered/deaths

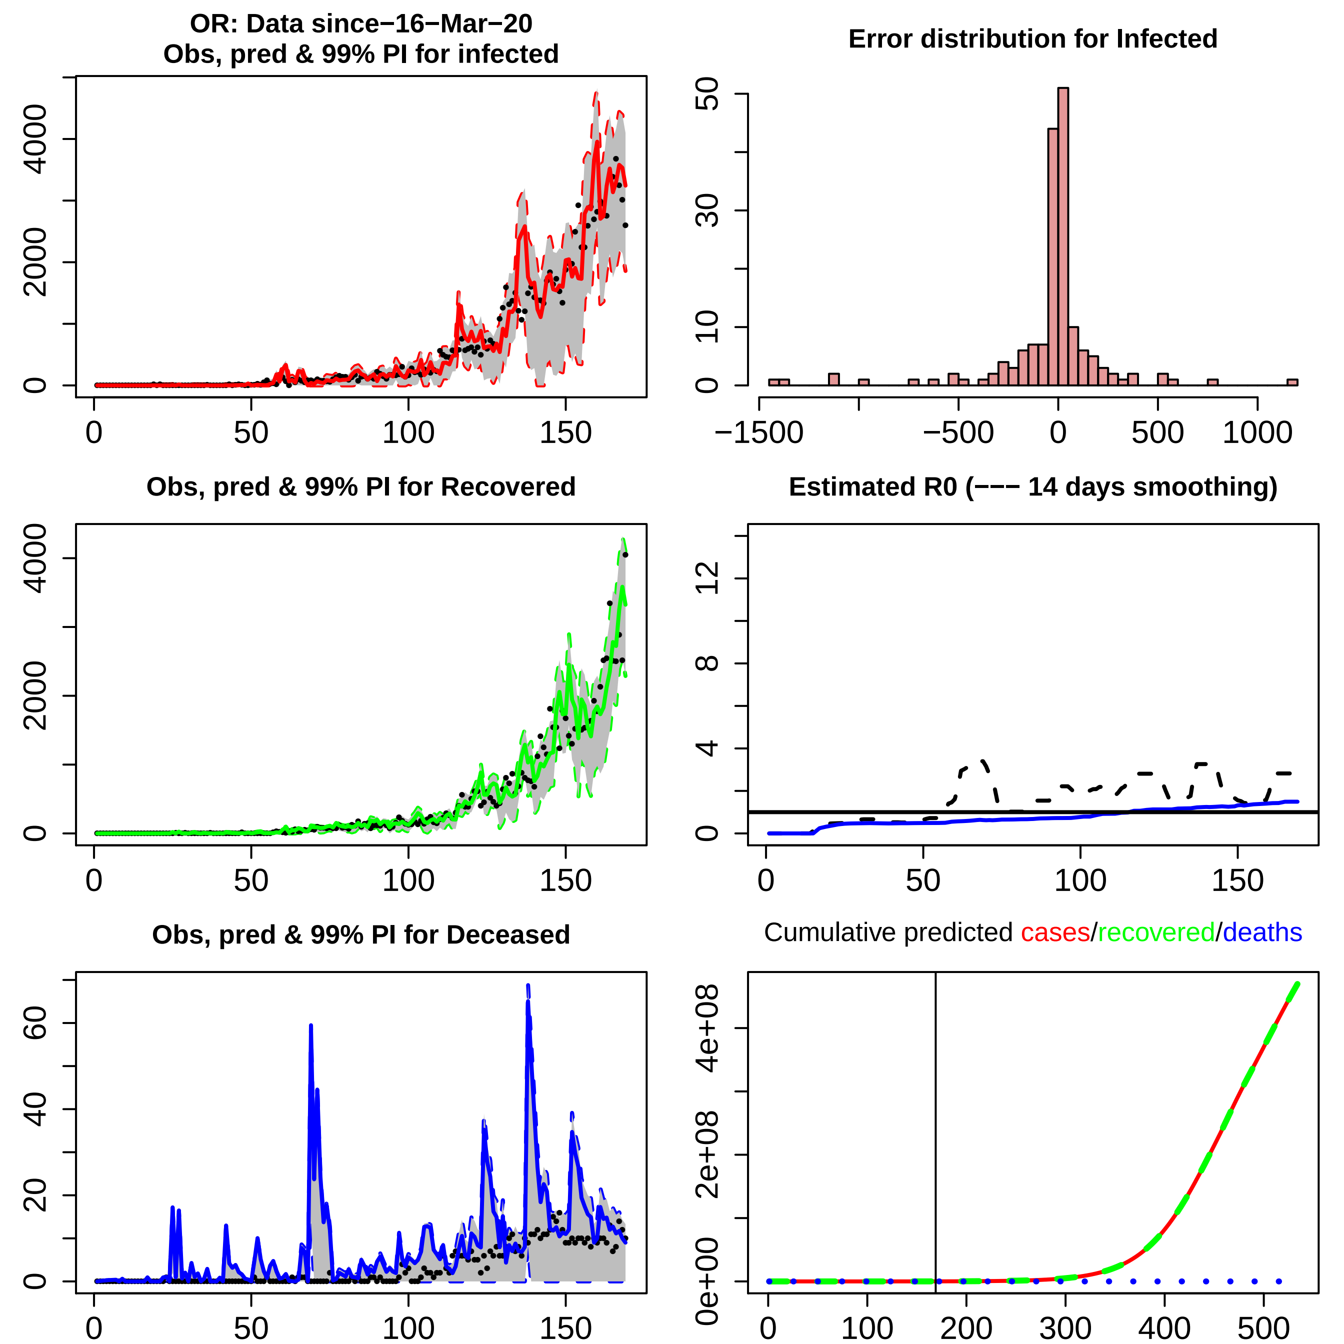

OR: Data since−16−Mar−20
Obs, pred & 99% PI for infected
Error distribution for Infected
Obs, pred & 99% PI for Recovered
Estimated R0 (−−− 14 days smoothing)
Obs, pred & 99% PI for Deceased
Cumulative predicted cases/recovered/deaths

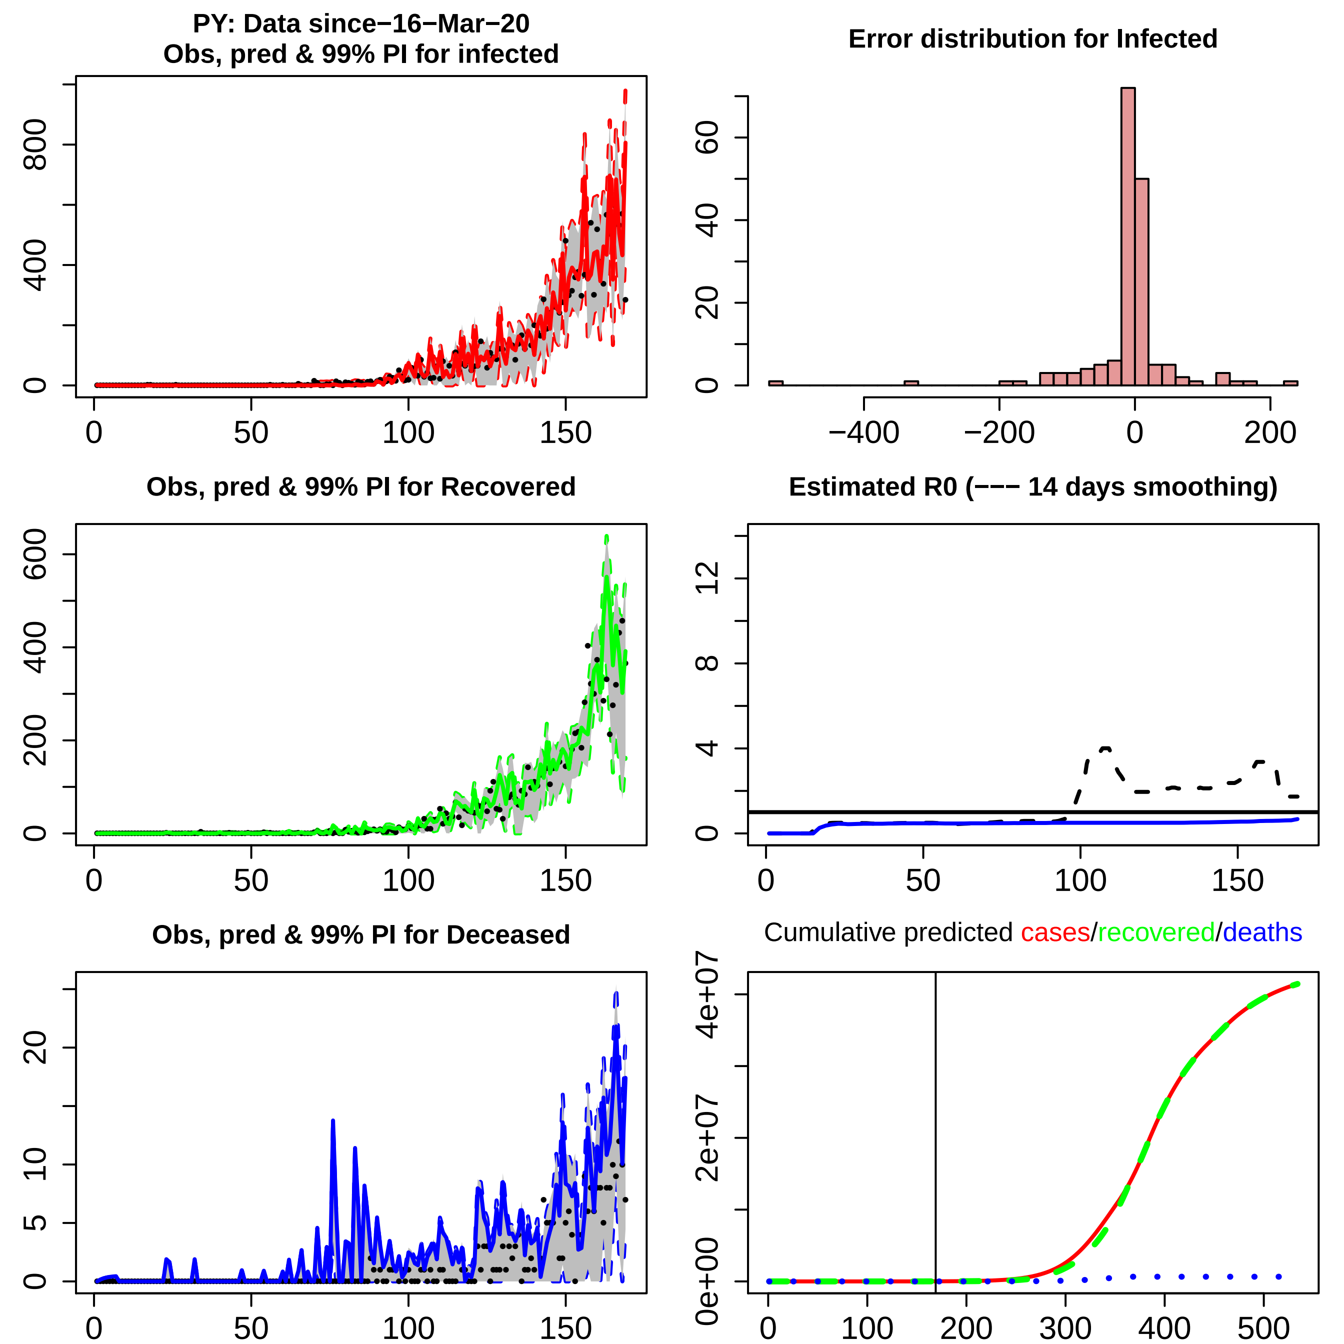

PY: Data since−16−Mar−20
Obs, pred & 99% PI for infected
Error distribution for Infected
Obs, pred & 99% PI for Recovered
Estimated R0 (−−− 14 days smoothing)
Obs, pred & 99% PI for Deceased
Cumulative predicted cases/recovered/deaths

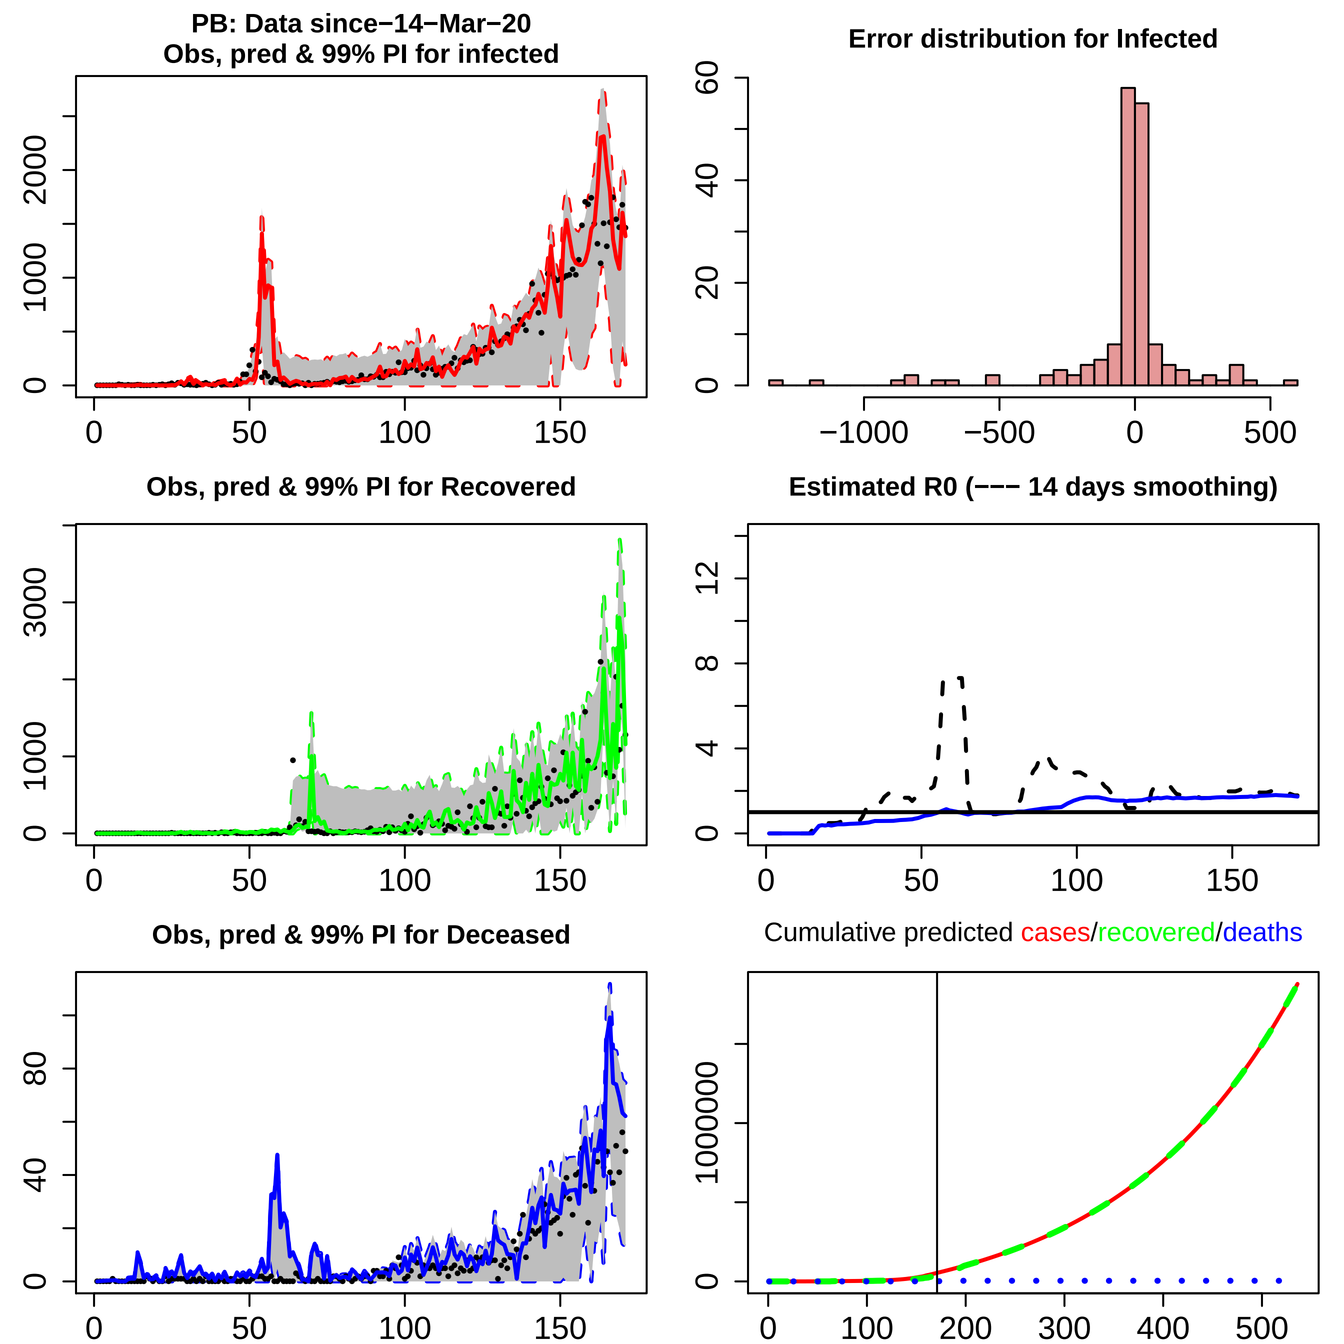
PB: Data since−14−Mar−20
Obs, pred & 99% PI for infected
Error distribution for Infected
Obs, pred & 99% PI for Recovered
Estimated R0 (−−− 14 days smoothing)
Obs, pred & 99% PI for Deceased
Cumulative predicted cases/recovered/deaths

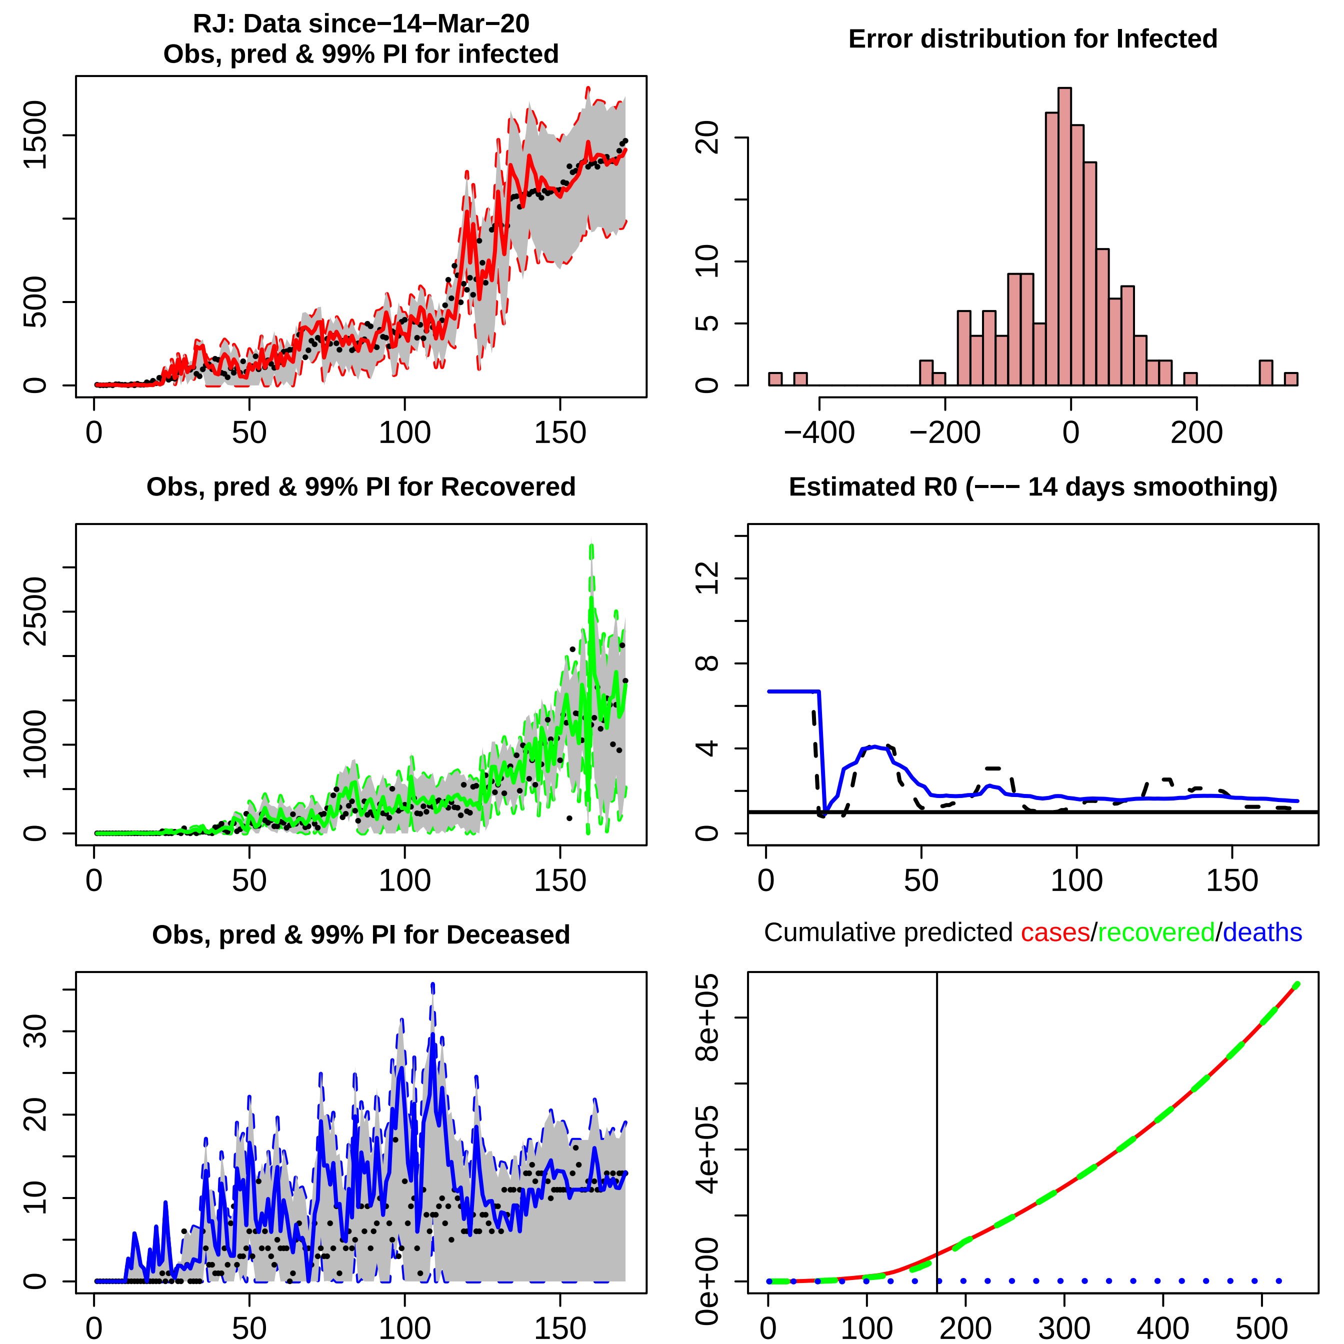
RJ: Data since−14−Mar−20
Obs, pred & 99% PI for infected
0
500
1500
0
50
100
150
Error distribution for Infected
0
5
10
20
−400
−200
0
200
Obs, pred & 99% PI for Recovered
0
1000
2500
0
50
100
150
Estimated R0 (−−− 14 days smoothing)
0
4
8
12
0
50
100
150
Obs, pred & 99% PI for Deceased
0
10
20
30
0
50
100
150
Cumulative predicted cases/recovered/deaths
0e+00
4e+05
8e+05
0
100
200
300
400
500

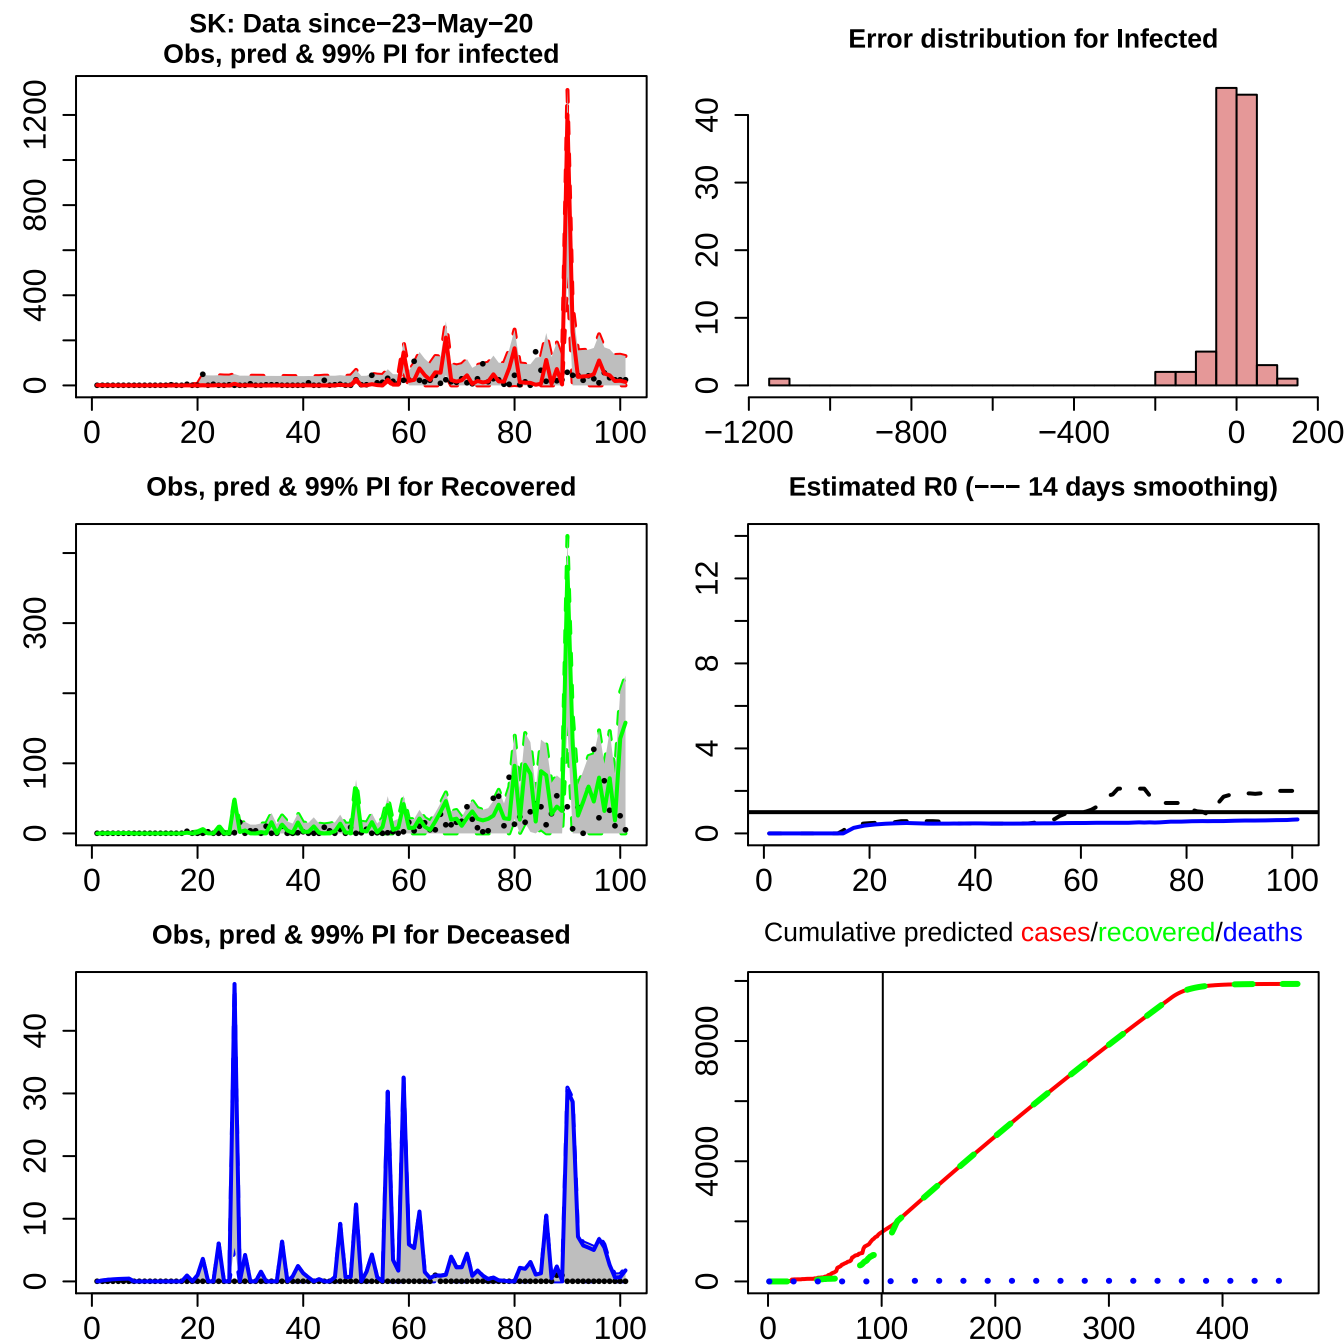

SK: Data since−23−May−20
Obs, pred & 99% PI for infected
Error distribution for Infected
Obs, pred & 99% PI for Recovered
Estimated R0 (−−− 14 days smoothing)
Obs, pred & 99% PI for Deceased
Cumulative predicted cases/recovered/deaths

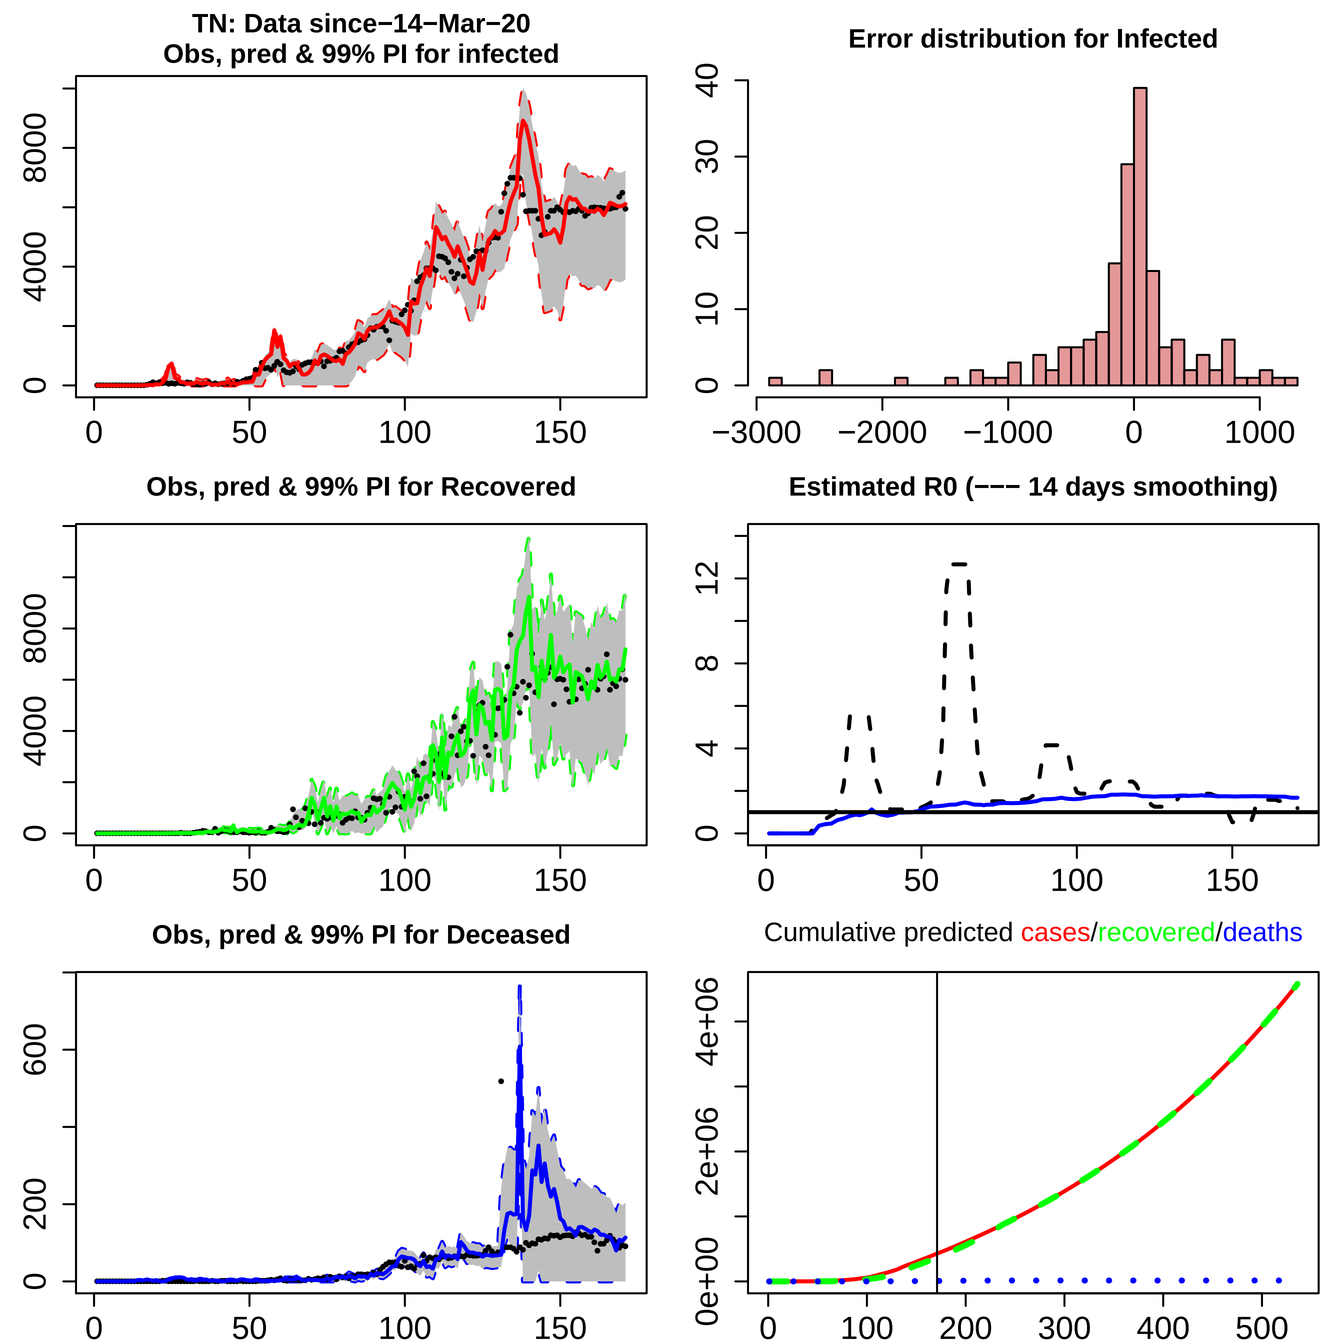
TN: Data since−14−Mar−20
Obs, pred & 99% PI for infected
Error distribution for Infected
Obs, pred & 99% PI for Recovered
Estimated R0 (−−− 14 days smoothing)
Obs, pred & 99% PI for Deceased
Cumulative predicted cases/recovered/deaths

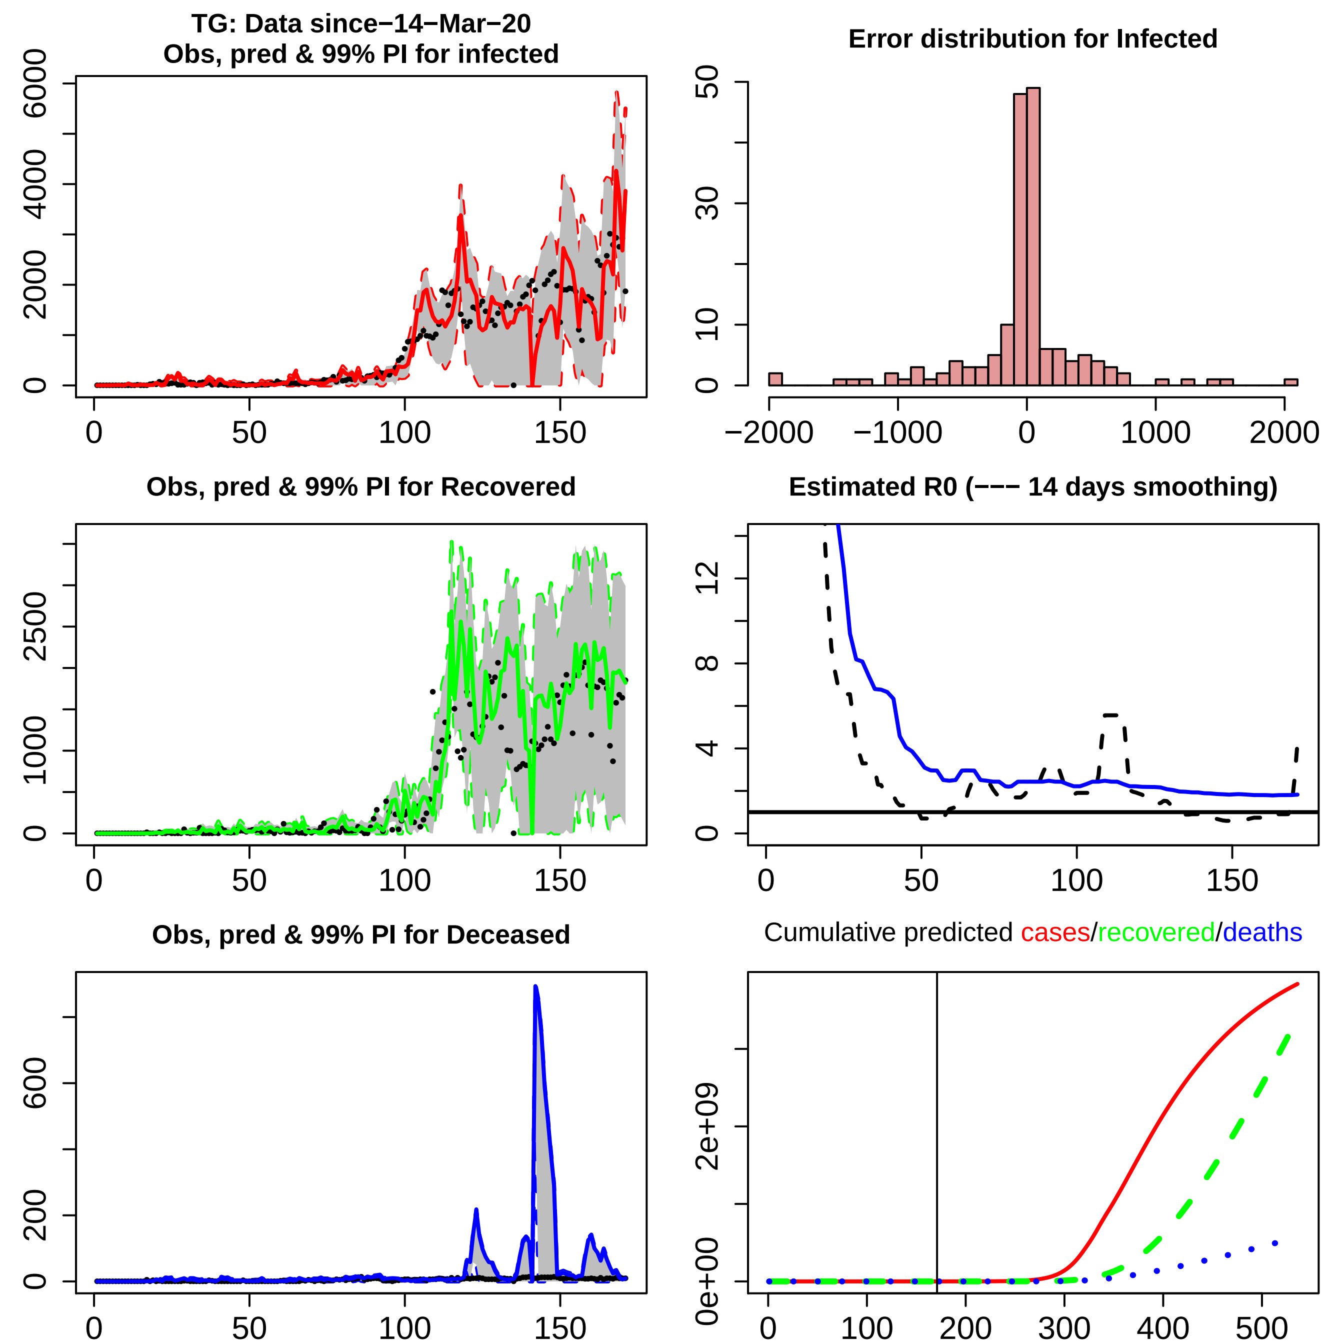
TG: Data since−14−Mar−20
Obs, pred & 99% PI for infected
Error distribution for Infected
Obs, pred & 99% PI for Recovered
Estimated R0 (−−− 14 days smoothing)
Obs, pred & 99% PI for Deceased
Cumulative predicted cases/recovered/deaths
0
2000
4000
6000
50
100
150
10
30
−2000
−1000
1000
500
2500
4
8
12
200
600
0e+00
2e+09
300
400

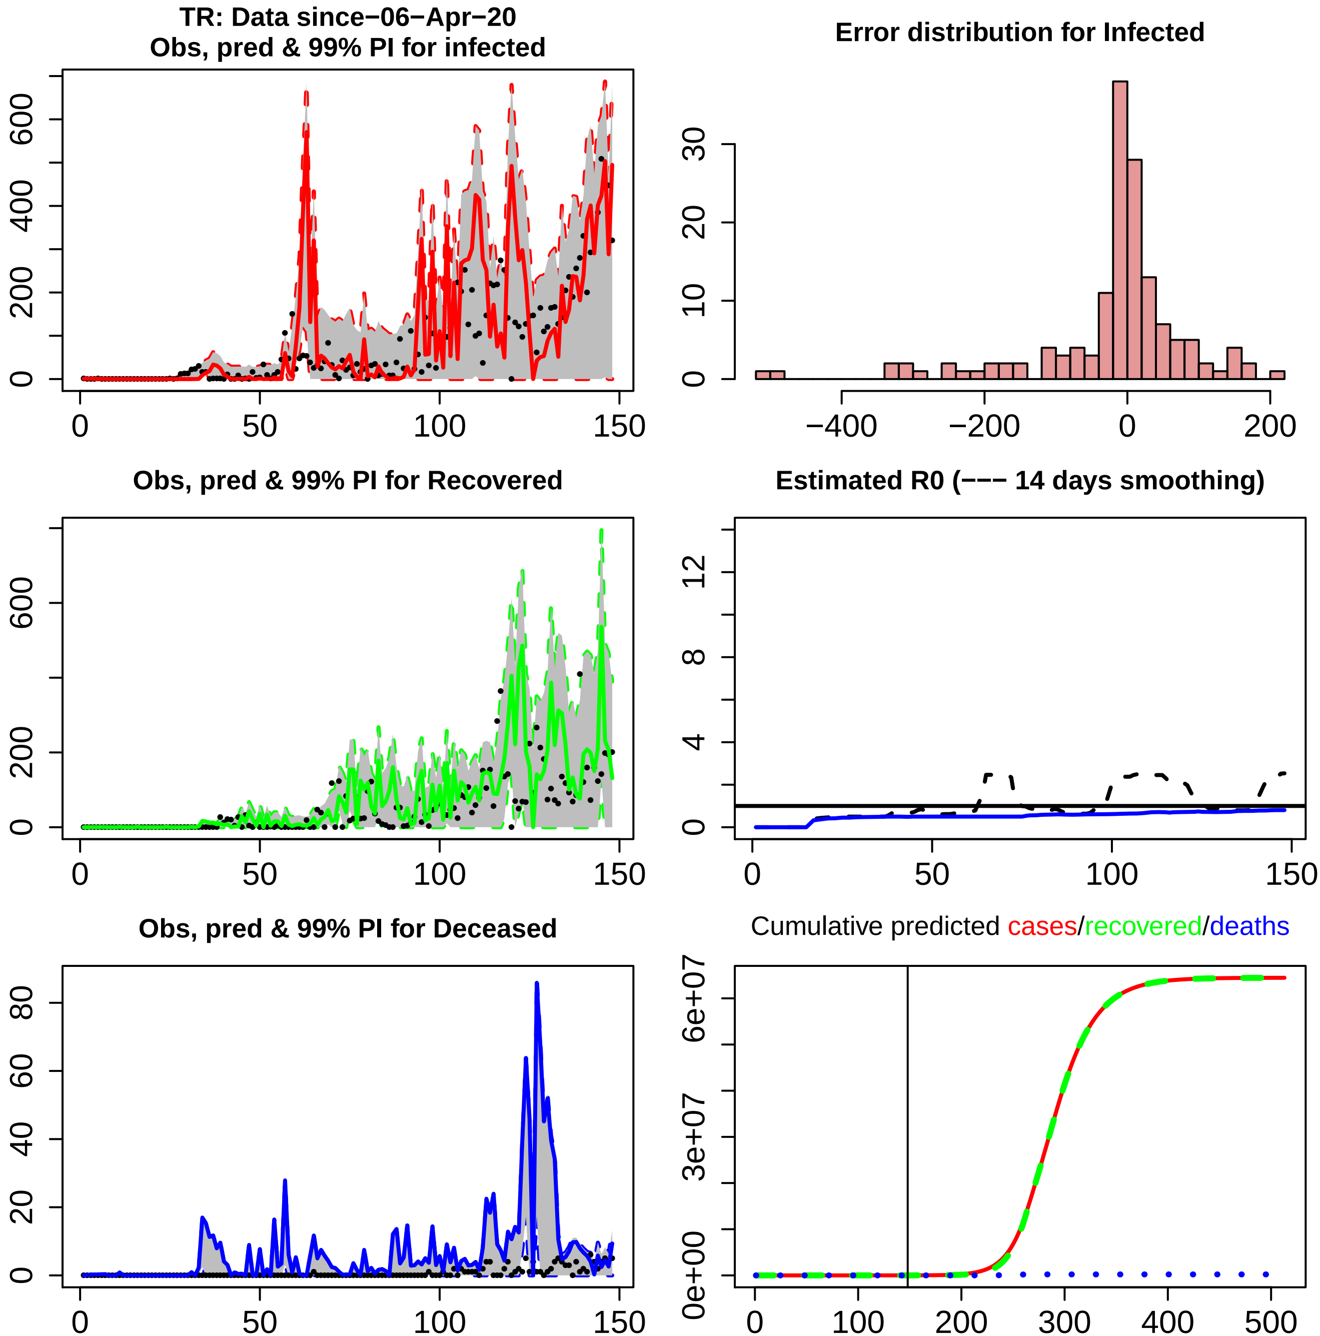
TR: Data since−06−Apr−20
Obs, pred & 99% PI for infected
Error distribution for Infected
Obs, pred & 99% PI for Recovered
Estimated R0 (−−− 14 days smoothing)
Obs, pred & 99% PI for Deceased
Cumulative predicted cases/recovered/deaths
0
200
400
600
50
100
150
10
20
30
−400
−200
4
8
12
0e+00
3e+07
6e+07
300
500
40
60
80

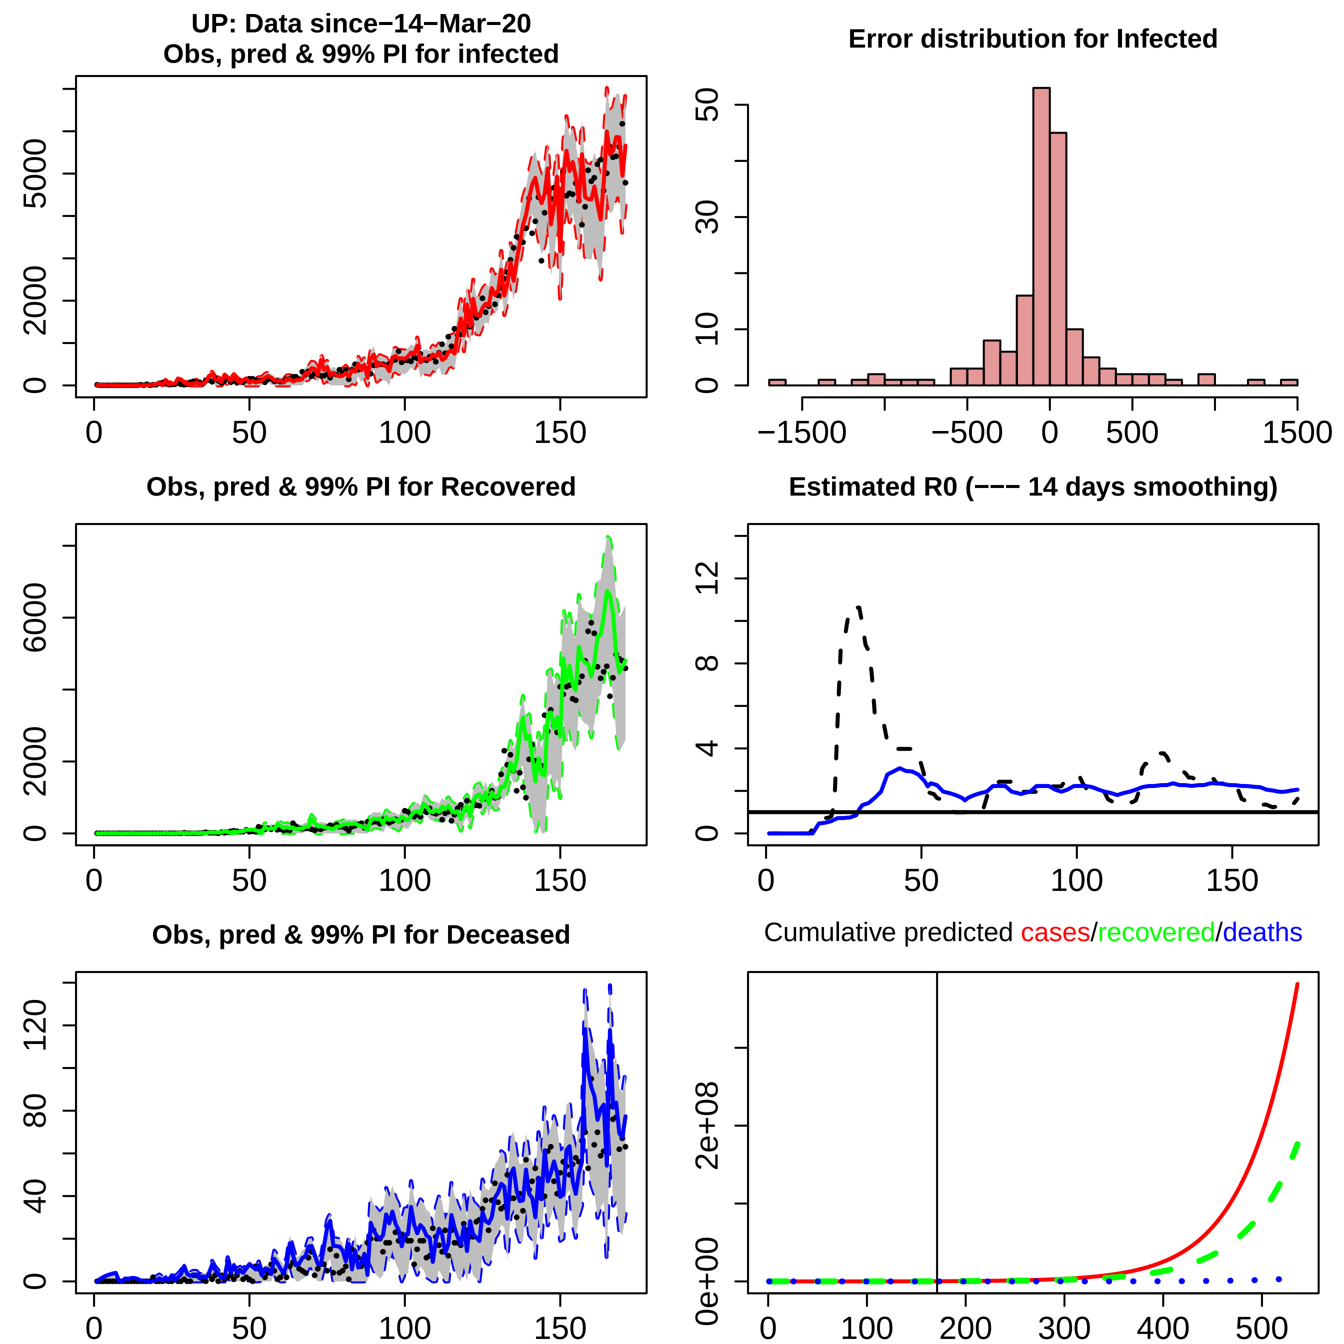

UP: Data since−14−Mar−20
Obs, pred & 99% PI for infected
Error distribution for Infected
Obs, pred & 99% PI for Recovered
Estimated R0 (−−− 14 days smoothing)
Obs, pred & 99% PI for Deceased
Cumulative predicted cases/recovered/deaths

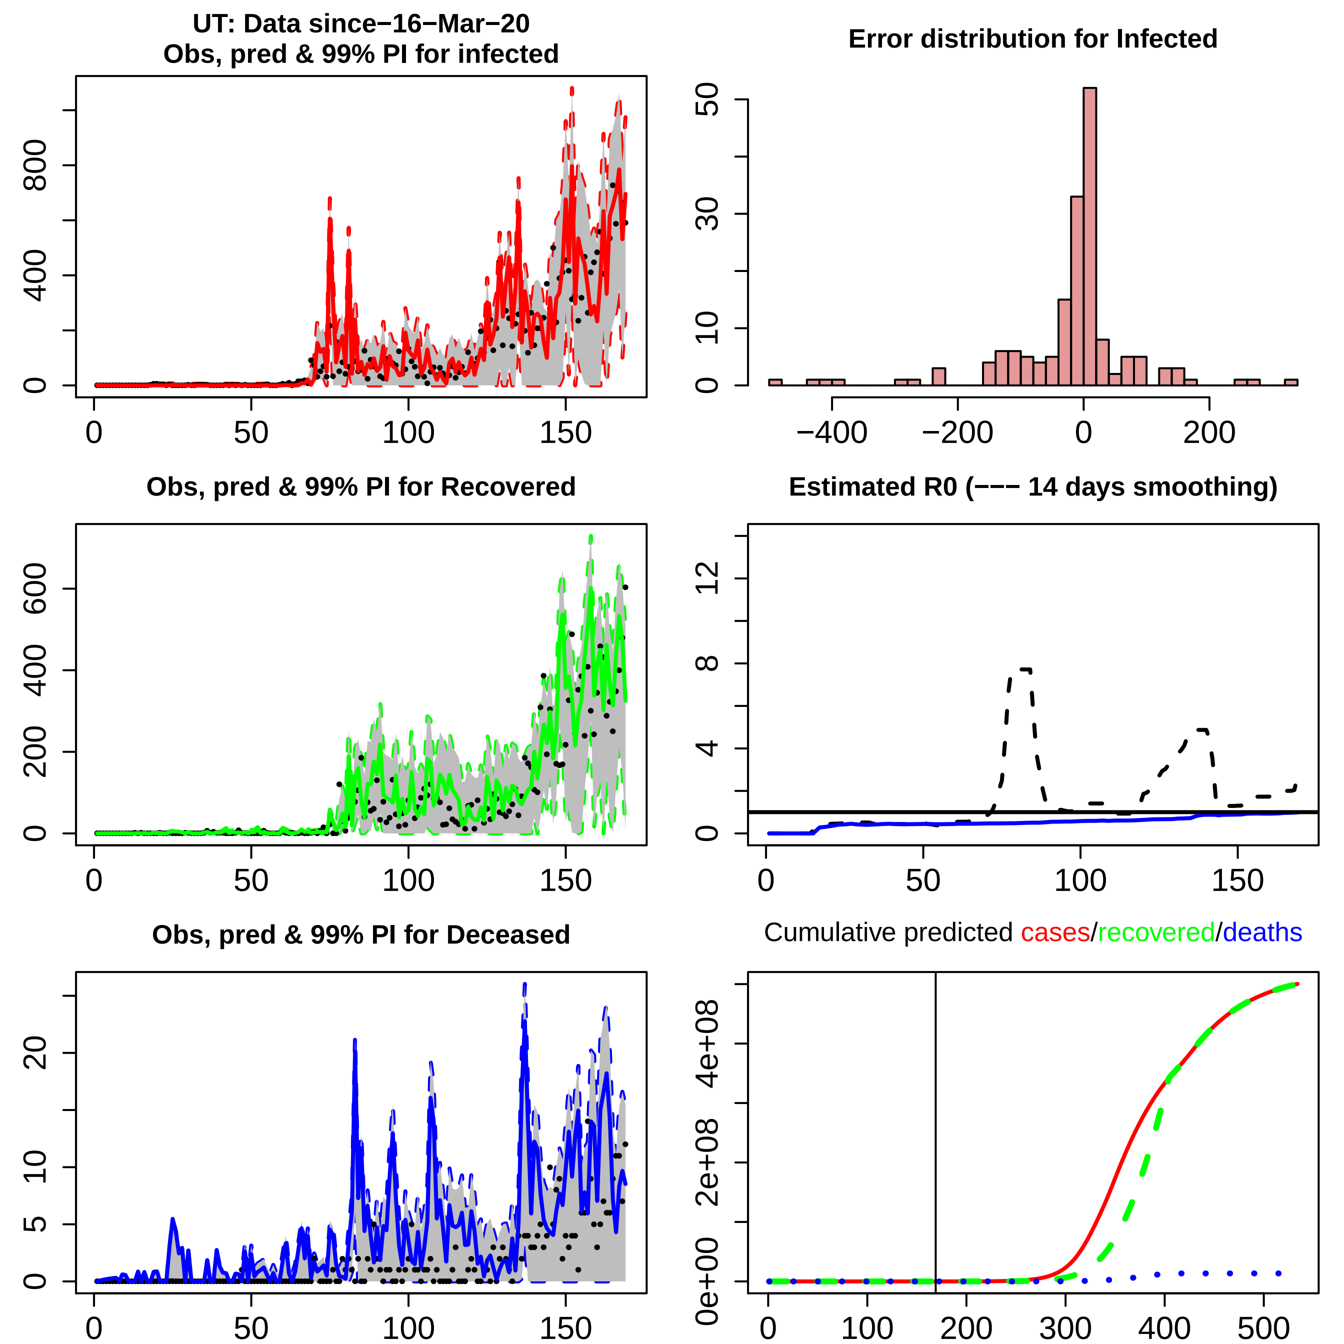
UT: Data since−16−Mar−20
Obs, pred & 99% PI for infected
Error distribution for Infected
Obs, pred & 99% PI for Recovered
Estimated R0 (−−− 14 days smoothing)
Obs, pred & 99% PI for Deceased
Cumulative predicted cases/recovered/deaths
0
400
800
50
100
150
10
30
−400
−200
200
600
4
8
12
5
20
0e+00
2e+08
4e+08
300
500

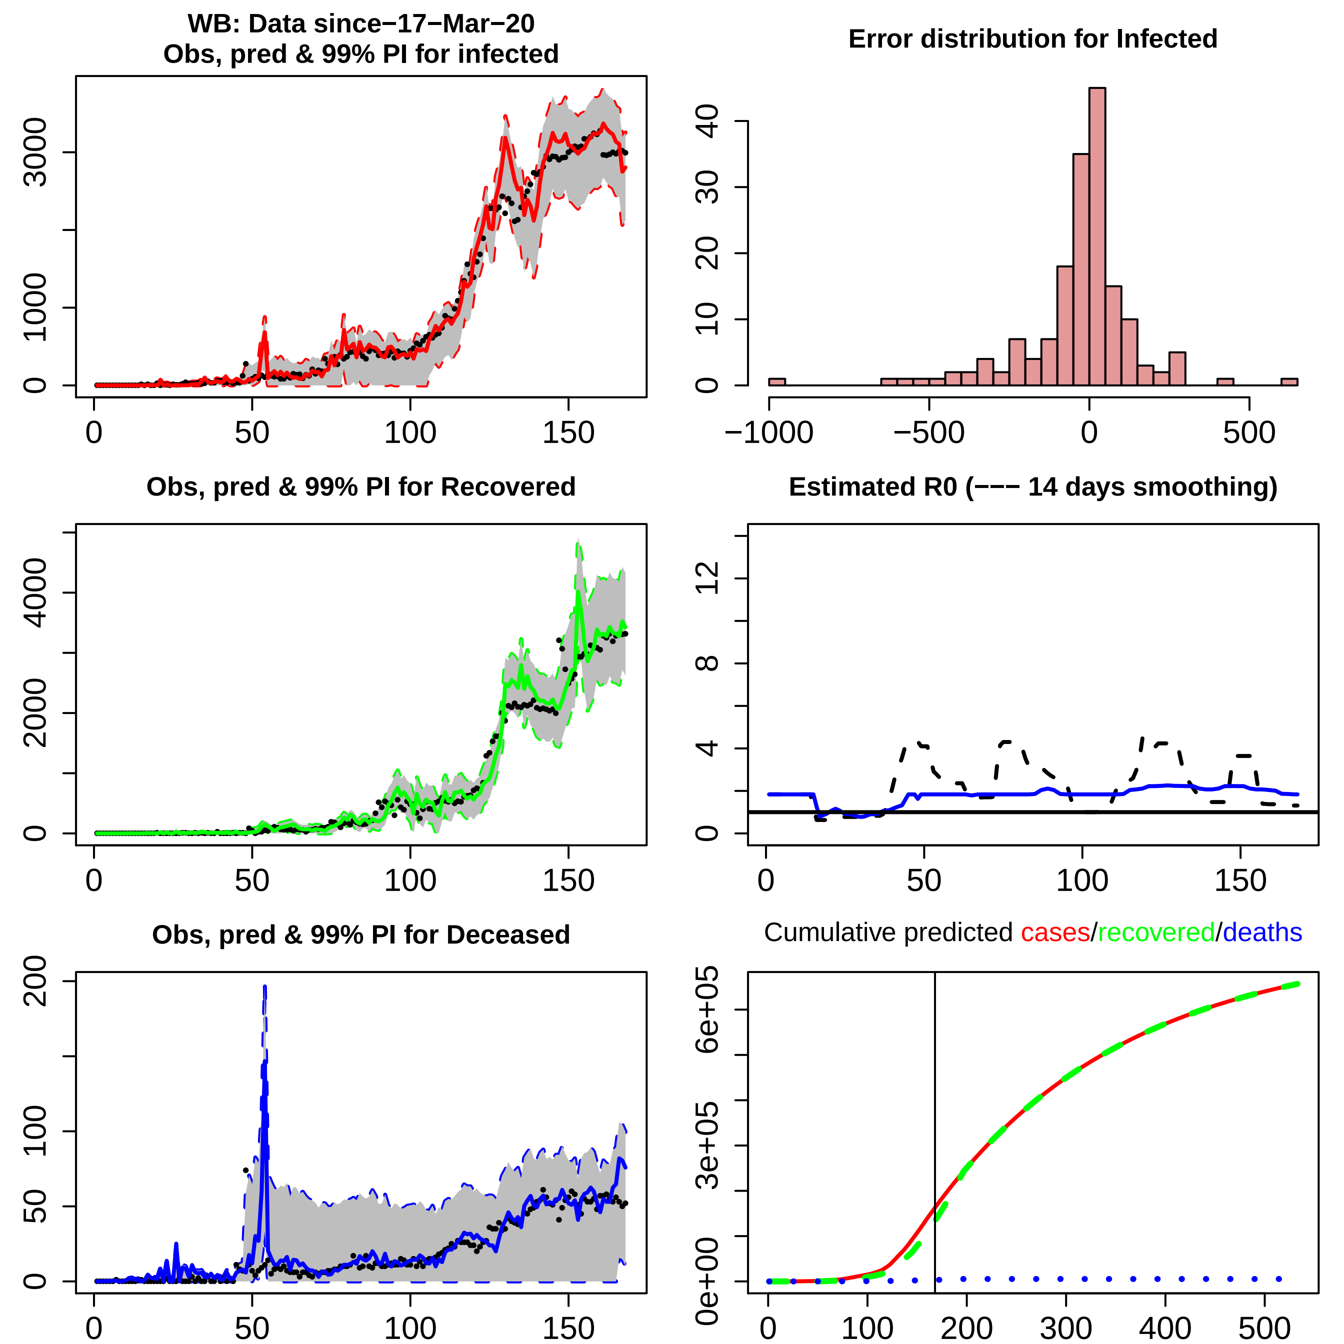
WB: Data since−17−Mar−20
Obs, pred & 99% PI for infected
0
1000
3000
0
50
100
150
Error distribution for Infected
0
10
20
30
40
−1000
−500
0
500
Obs, pred & 99% PI for Recovered
0
2000
4000
0
50
100
150
Estimated R0 (−−− 14 days smoothing)
0
4
8
12
0
50
100
150
Obs, pred & 99% PI for Deceased
0
50
100
200
0
50
100
150
Cumulative predicted cases/recovered/deaths
0e+00
3e+05
6e+05
0
100
200
300
400
500
